# Supplementary material for: Learning to represent signals spike by spike
Source: arXiv:1703.03777 ancillary file (2017-03-16)
Supplement: Supplementary file 1 [file SI.pdf]

# Supplementary Material

## Learning to represent signals spike by spike

The supplementary material is structured as follows: In section 1 we describe the spiking recurrent neural networks that we are using throughout the paper, and we review the connectivity patterns of the networks that optimally encode the input signals in their spike trains. We then discuss the problem of learning the connectivity of the respective optimal networks in section 2 and provide the core intuitions on learning in section 3, namely, that the tight balance between excitatory and inhibitory currents is the key signature of the optimal networks that needs to be learnt. In section 4 we then derive the voltage-based synaptic plasticity rules for the feedforward and recurrent connections that are used in the main paper, and we discuss their mathematical properties. In section 5 we apply these learning rules to the full E/I network. Finally, in the last section, we provide all simulation parameters as well as pseudo-code.

## Contents

|          |                                                                                   |           |
|----------|-----------------------------------------------------------------------------------|-----------|
| <b>1</b> | <b>Spiking recurrent neural networks</b>                                          | <b>2</b>  |
| 1.1      | Inputs and outputs                                                                | 2         |
| 1.2      | Voltage dynamics                                                                  | 3         |
| 1.3      | Voltage dynamics without interneurons                                             | 4         |
| 1.4      | Readouts and objectives                                                           | 4         |
| 1.5      | The optimal decoder                                                               | 6         |
| 1.6      | The optimal decoder under length constraints                                      | 6         |
| 1.7      | The connectivity and thresholds of the optimal network                            | 7         |
| 1.8      | The cost-term revisited                                                           | 8         |
| <b>2</b> | <b>The learning problem</b>                                                       | <b>9</b>  |
| 2.1      | Classical approaches to learning in recurrent neural networks                     | 9         |
| 2.2      | The efficient coding objective                                                    | 10        |
| 2.3      | The problem of learning the synaptic weights                                      | 11        |
| 2.4      | The problem of the appropriate decoder scale                                      | 11        |
| <b>3</b> | <b>The core intuitions behind learning</b>                                        | <b>11</b> |
| 3.1      | Error-driven coding                                                               | 12        |
| 3.2      | The four conditions of learning                                                   | 12        |
| 3.3      | Condition 1: Recurrent weights learn to balance feedforward inputs spike by spike | 13        |
| 3.4      | Condition 2: Spike-by-spike balance results in error-driven coding                | 15        |
| 3.5      | Interlude: The importance of quadratic costs                                      | 16        |
| 3.6      | Condition 3: Feedforward weights learn to mimic the decoder                       | 16        |

|          |                                                                    |           |
|----------|--------------------------------------------------------------------|-----------|
| 3.7      | Condition 4: Learning rules minimize loss function . . . . .       | 17        |
| 3.8      | Conclusions and biological realism reconsidered . . . . .          | 18        |
| <b>4</b> | <b>The Voltage-based learning rules . . . . .</b>                  | <b>18</b> |
| 4.1      | Recurrent weights: Learning in the absence of cost terms . . . . . | 18        |
| 4.2      | Recurrent weights: Fixed point analysis . . . . .                  | 20        |
| 4.3      | Recurrent weights: Convergence proof . . . . .                     | 21        |
| 4.4      | Recurrent weights: Learning with L2 costs . . . . .                | 22        |
| 4.5      | Feedforward weights: Learning rule . . . . .                       | 23        |
| 4.6      | Feedforward weights: Fixed-point analysis . . . . .                | 23        |
| 4.7      | L1 cost and the scaling problem . . . . .                          | 24        |
| 4.8      | Non-whitened inputs . . . . .                                      | 26        |
| 4.9      | Simplifying assumptions for the main paper . . . . .               | 27        |
| <b>5</b> | <b>Learning in the E/I network . . . . .</b>                       | <b>28</b> |
| <b>6</b> | <b>Robustness of learning . . . . .</b>                            | <b>29</b> |
| <b>7</b> | <b>Learning a Speech signal, Supplementary results . . . . .</b>   | <b>30</b> |
| <b>8</b> | <b>Numerical Simulations . . . . .</b>                             | <b>30</b> |
| 8.1      | Network Dynamics . . . . .                                         | 30        |
| 8.2      | Initialization . . . . .                                           | 31        |
| 8.3      | Tuning Curves . . . . .                                            | 31        |
| 8.4      | Fano Factor and Coefficient of Variation . . . . .                 | 35        |
| 8.5      | Learning the Speech Signal . . . . .                               | 35        |

# 1 Spiking recurrent neural networks

In this section, we describe the network of integrate-and-fire neurons whose synaptic weights we will learn. We furthermore introduce an optimality criterion that we will use to define an ‘optimal’ spiking neural network, whose specific connectivity structure will provide the target of learning. We largely follow the derivations of [1, 2].

## 1.1 Inputs and outputs

We consider a recurrent neural network with  $N_E$  excitatory and  $N_I$  inhibitory neurons (compare Figure 1Ai in the main paper). The network receives a set of time-varying inputs  $\mathbf{c}(t) = (c_1(t), c_2(t), \dots, c_I(t))$  and produces a set of spike train outputs from the excitatory population,  $\mathbf{o}^E(t) = (o_1^E(t), o_2^E(t), \dots, o_{N_E}^E(t))$ .<sup>1</sup> Each spike train is as a sum of Dirac delta functions,  $o(t) = \sum_{t_k} \delta(t - t_k)$ , where  $t_k$  are the spike times.

---

<sup>1</sup>In general, we will use bold-faced letters to indicate vectors or matrices, and italic letters to indicate scalar variables.

We furthermore define filtered versions of the input and output signals. First, the filtered input signal,  $\mathbf{x}(t)$ , is given by

$$\dot{\mathbf{x}}(t) = -\lambda \mathbf{x}(t) + \mathbf{c}(t), \quad (\text{S.1})$$

and the filtered spike trains of the excitatory neurons are given by

$$\dot{\mathbf{r}}^E(t) = -\lambda \mathbf{r}^E(t) + \mathbf{o}^E(t). \quad (\text{S.2})$$

Here, the parameter  $\lambda$  sets the decay rate of the respective variables. We note that for slowly changing signals,  $\mathbf{x}(t)$  and  $\mathbf{c}(t)$  are just scaled versions of each other. This is the scenario most applicable to our work, and we therefore refer to both variables as ‘input signals’. Indeed, in the main text we did not distinguish between  $\mathbf{c}(t)$  and  $\mathbf{x}(t)$ , but will do so here to be mathematically exact. We assume that these input signals are distributed according to some distribution  $q(\mathbf{x})$ . Throughout the first part of the supplementary information (SI), we will assume that this distribution is ‘white’, i.e., that its covariance matrix is the identity.

Each filtered spike trains can be viewed as a sum over postsynaptic potentials. We will sometimes refer to these filtered spike trains as ‘instantaneous firing rates’ or simply ‘firing rates’, even though, strictly speaking, the variables  $r_i^E(t)$  have units of firing rates scaled by a factor  $1/\lambda$ . We note that this definition slightly deviates from [1]. The spike trains of the inhibitory interneurons are not considered to be part of the output. We will simply write  $\mathbf{o}^I(t)$  for the vector of these spike trains, and  $\mathbf{r}^I(t)$  for the respective filtered versions. Since there are  $N_I$  inhibitory neurons, both vectors are  $N_I$ -dimensional.

## 1.2 Voltage dynamics

We assume that the membrane voltages of both the excitatory and inhibitory neurons follow the dynamics of current-based, leaky integrate-and-fire neurons. Specifically, the voltage  $V_n^E$  of the  $n$ -th excitatory neuron is given by

$$\dot{V}_n^E(t) \equiv \frac{\partial V_n^E}{\partial t} = -\lambda V_n^E(t) + \mathbf{F}_n^E \cdot \mathbf{c}(t) + \mathbf{\Omega}_n^{EE} \cdot \mathbf{o}^E(t) + \mathbf{\Omega}_n^{EI} \cdot \mathbf{o}^I(t) + \sigma\eta(t), \quad (\text{S.3})$$

where  $\mathbf{F}_n^E$  are the feedforward weights of neuron  $n$ ,  $\mathbf{\Omega}_n^{EE}$  are the weights of the recurrent excitatory inputs,  $\mathbf{\Omega}_n^{EI}$  are the weights of the recurrent inhibitory inputs, and  $\sigma\eta(t)$  is a noise term. The multiplication sign ‘ $\cdot$ ’ denotes the inner product or dot product. We generally assume that the feedforward weights can be either excitatory or inhibitory, meaning that individual elements of  $\mathbf{F}_n^E$  can be either positive or negative. The elements of  $\mathbf{\Omega}_n^{EI}$  are assumed to be negative and the elements of  $\mathbf{\Omega}_n^{EE}$  are assumed to be positive, with one exception: the self-connection weight  $\Omega_{nn}^{EE}$  is assumed to be negative, as it determines the neuron’s reset potential after a spike. Whenever the neuron hits a threshold,  $T_n^E$ , it fires a spike and resets its own voltage. In other words, we have included the reset of the integrate-and-fire neuron in its self-connection for mathematical convenience. After each spike, the voltage is therefore reset to  $V_n^E \rightarrow T_n^E + \Omega_{nn}^{EE}$ , where  $\Omega_{nn}^{EE}$  is a negative number.

Similarly, the membrane voltage  $V_n^I$  of the  $n$ -th inhibitory neuron follows the dynamics

$$\dot{V}_n^I(t) \equiv \frac{\partial V_n^I}{\partial t} = -\lambda V_n^I(t) + \mathbf{\Omega}_n^{IE} \cdot \mathbf{o}^E(t) + \mathbf{\Omega}_n^{II} \cdot \mathbf{o}^I(t) + \sigma\eta(t), \quad (\text{S.4})$$

where  $\mathbf{\Omega}_n^{IE}$  are the recurrent weights from the excitatory population and  $\mathbf{\Omega}_n^{II}$  are the recurrent weights from the inhibitory population. The thresholds are given by  $T_n^I$  and the reset is contained in the element  $\Omega_{nn}^{II}$  of the recurrent inhibitory input.

### 1.3 Voltage dynamics without interneurons

To develop the learning rules for this network, it will prove quite useful to start with a simpler network in which we ignore the constraints imposed on biological networks due to Dale’s law, i.e., due to the split of excitation and inhibition into separate pools of neurons. To this end, we will defer the treatment of the full E/I network to section 5 and omit the inhibitory interneurons from now on by allowing direct inhibition between the excitatory neurons. We can then drop all E/I subscripts and simplify the dynamics of the membrane voltage,

$$\dot{V}_n(t) = -\lambda V_n(t) + \mathbf{F}_n^\top \mathbf{c}(t) + \mathbf{\Omega}_n^\top \mathbf{o}(t) \quad (\text{S.5})$$

where the neuron index  $n$  runs from  $1 \dots N$  (with  $N = N_E$ ) and the recurrent weights  $\mathbf{\Omega}_n \in \mathbb{R}^N$  can be both excitatory or inhibitory. We also left out the noise term, since it will essentially be irrelevant for the derivation of the learning rules. The treatment of the full E/I network can be found in section 5. For notational convenience, we will furthermore write all inner products as matrix products, so that  $\mathbf{F}_n \cdot \mathbf{c}(t) = \mathbf{F}_n^\top \mathbf{c}(t)$  etc.

The synaptic weights of the individual neurons can be combined to yield the connectivity matrices of the network. Throughout the SI, we define the  $N \times I$  matrix of feedforward weights as  $\mathbf{F} = [\mathbf{F}_1, \mathbf{F}_2, \dots, \mathbf{F}_N]^\top$  and the  $N \times N$  matrix of recurrent weights as  $\mathbf{\Omega} = [\mathbf{\Omega}_1, \dots, \mathbf{\Omega}_N]^\top$ . This allows us to write the dynamics of the whole network in the compact form

$$\dot{\mathbf{V}}(t) = -\lambda \mathbf{V}(t) + \mathbf{F} \mathbf{c}(t) + \mathbf{\Omega} \mathbf{o}(t),$$

where  $\mathbf{V}$  is simply the  $N$ -dimensional vector of all voltages. Finally, we can formally integrate the differential equation, using (S.1) and (S.2), to obtain

$$\mathbf{V}(t) = \mathbf{F} \mathbf{x}(t) + \mathbf{\Omega} \mathbf{r}(t). \quad (\text{S.6})$$

Note that this integration does not constitute an explicit solution to the differential equation, since the instantaneous firing rates,  $\mathbf{r}(t)$ , appear on the r.h.s. However, the integration highlights the particular relation between the voltages and the filtered spike trains, which will become useful further below.

### 1.4 Readouts and objectives

The network receives the time-varying input signals,  $\mathbf{x}(t)$ , and generates a set of output spike trains,  $\mathbf{o}(t)$ . We will assume that a downstream area will seek to construct an estimate  $\hat{\mathbf{x}}(t)$  of the input signal from a simple weighted sum of

the filtered output spike trains,<sup>2</sup>

$$\begin{aligned}\hat{\mathbf{x}} &= \mathbf{D}\mathbf{r} \\ &= \sum_{n=1}^{N_E} \mathbf{D}_n r_n\end{aligned}\tag{S.7}$$

where  $\mathbf{D}$  is an  $I \times N_E$  matrix of decoder weights, and  $\mathbf{D}_n$  are the columns of this matrix. The vector  $\mathbf{D}_n$  summarizes the contribution of neuron  $n$  to the reconstruction of the signal.<sup>3</sup> For future reference, we note that we can use (S.2) to obtain a differential equation for this readout,

$$\dot{\hat{\mathbf{x}}} = -\lambda \hat{\mathbf{x}} + \mathbf{D}\mathbf{o}.$$

We can measure the quality of any readout by averaging its performance over a time interval  $T$ . To denote time averages of a quantity  $z(t)$ , we will use angular brackets so that  $\langle z(t) \rangle_t = \frac{1}{T} \int_0^T z(t) dt$ . With this in mind, we define the following loss function,

$$\begin{aligned}L &= \langle \ell(t) \rangle_t \\ &\equiv \left\langle \|\mathbf{x}(t) - \hat{\mathbf{x}}(t)\|^2 + C(\mathbf{r}(t)) \right\rangle_t\end{aligned}$$

where the first term inside the brackets is a quadratic measure of the reconstruction error, the second term is a cost term on the firing rates. If the time interval  $T$  over which this loss is averaged is large compared to the time-scale of the input, then the distribution of inputs  $\mathbf{c}$  during this interval is approximately the same as the true input distribution  $q(\mathbf{c})$ . Hence, for large  $T$  we essentially sample the loss evenly over the distribution  $q(\mathbf{c})$  of all possible inputs  $\mathbf{c}$  (and hence over the distribution of input signals  $q(\mathbf{x})$ , since the signals  $\mathbf{x}$  are filtered versions of  $\mathbf{c}$ ). To denote expectation values of a quantity  $z(\mathbf{x})$  with respect to the distribution  $q(\mathbf{x})$ , we will again use angular brackets, writing  $\langle z(\mathbf{x}) \rangle_{q(\mathbf{x})} = \int d\mathbf{x} q(\mathbf{x}) z(\mathbf{x})$ . Accordingly, we can rewrite (S.8) as an estimate of the expected loss over the inputs,<sup>4</sup>

$$\begin{aligned}L &= \langle \ell(\mathbf{x}) \rangle_{q(\mathbf{x})} \\ &= \left\langle \|\mathbf{x} - \hat{\mathbf{x}}\|^2 + C(\mathbf{r}) \right\rangle_{q(\mathbf{x})}.\end{aligned}\tag{S.8}$$

For ease of notation we will typically suppress the difference between these two formulations and simply use angular brackets,  $\langle z \rangle$ , to denote averaging of the variable  $z$  over either time or input signals. Similarly, we will write

$$\ell = \|\mathbf{x} - \hat{\mathbf{x}}\|^2 + C(\mathbf{r})\tag{S.9}$$

<sup>2</sup>Please note that we will generally drop the explicit notion of time-dependence to streamline the presentation, and so we here write  $\hat{\mathbf{x}}$  instead of  $\hat{\mathbf{x}}(t)$  and  $\mathbf{r}$  instead of  $\mathbf{r}(t)$ .

<sup>3</sup>Please note that  $\mathbf{D}_n$  denotes a *column* of the decoder matrix  $\mathbf{D}$  whereas  $\mathbf{F}_n$ , for instance, denotes a *row* of the matrix of excitatory feedforward weights. Nonetheless, all vectors, including these two, are assumed to be column vectors.

<sup>4</sup>We previously assumed that the distribution  $q(\mathbf{x})$  is white, i.e., its covariance matrix is the identity. For non-white signals, it is advantageous to modify the definition of the loss, and we will discuss this more general case in section 4.8.

to refer either to the time-dependent loss  $\ell(t)$  or the signal-dependent loss  $\ell(\mathbf{x})$ .

The cost term,  $C(\mathbf{r})$ , allows us to assign a ‘cost’ to the representation (in terms of filtered spike trains) chosen by a particular network. Typical choices for the cost-term are  $C(\mathbf{r}) = \sum_i r_i^2 = \|\mathbf{r}\|^2$  or  $C(\mathbf{r}) = \sum_i |r_i| = \|\mathbf{r}\|_1$ . (We will discuss the rationale for these choices in section 1.8.) For concreteness, we adopt a linear sum of the two, but many results and intuitions directly generalize to other cost functions. The objective (S.9) then reads

$$\ell = \|\mathbf{x} - \hat{\mathbf{x}}\|^2 + \mu \|\mathbf{r}\|^2 + \nu \|\mathbf{r}\|_1. \quad (\text{S.10})$$

## 1.5 The optimal decoder

The cost function not only allows us to define the quality of a particular reconstruction,  $\hat{\mathbf{x}} = \mathbf{D}\mathbf{r}$ , but it also allows us to determine the best possible decoder  $\mathbf{D}$  for a given network. The corresponding optimization problem is identical to linear regression. Taking the derivative of (S.8) with respect to  $\mathbf{D}$ , we have

$$\frac{\partial L}{\partial \mathbf{D}} = -2 \langle (\mathbf{x} - \hat{\mathbf{x}}) \mathbf{r}^\top \rangle,$$

which we can set to zero to obtain the well-known linear regression solution,

$$\mathbf{D} = \langle \mathbf{x} \mathbf{r}^\top \rangle \langle \mathbf{r} \mathbf{r}^\top \rangle^{-1}.$$

For each particular network architecture with feedforward weights  $\mathbf{F}$  and recurrent weights  $\mathbf{\Omega}$ , we can employ this formula to find the respective optimal decoder. Indeed, we used this formula in Figure 2 in the main text, where we compare the reconstructed signal with the input signal both for the the unlearned network and for the learnt network.

## 1.6 The optimal decoder under length constraints

The (optimal) decoder will be an important conceptual quantity for the learning rules of the spiking network. In that context, however, the optimal decoder will be constrained to be of a particular length. While the necessity of this constraint will only become clear below, we here describe the corresponding optimization problem for future reference. (This subsection can also be skipped on first reading.)

Specifically, we will constrain the neurons’ individual contributions to the readout,  $\mathbf{D}_n$ , to be of a certain length. Using a set of Lagrangian multipliers  $\lambda_n$ , we simply add these length constraints to the mean square error of the reconstruction to obtain the modified loss function <sup>5</sup>

$$L = \langle \|\mathbf{x} - \hat{\mathbf{x}}\|^2 \rangle + \sum_{n=1}^{N_E} \lambda_n (\|\mathbf{D}_n\|^2 - a_n),$$

where  $a_n$  specifies the length of the  $n$ -th decoder  $\mathbf{D}_n$ . Taking the derivative of the loss with respect to  $\mathbf{D}_n$  (and remembering that  $\hat{\mathbf{x}} = \sum_n \mathbf{D}_n r_n$ ) yields

$$\frac{\partial L}{\partial \mathbf{D}_n} = -2 \langle (\mathbf{x} - \hat{\mathbf{x}}) r_n \rangle + 2\lambda_n \mathbf{D}_n.$$

---

<sup>5</sup>Note that we leave out the cost term  $C(\mathbf{r})$  since it do not depend on the decoder.

In turn, we can set the derivative to zero to find the minimum of the loss function. An insightful *implicit* solution is found by writing

$$\mathbf{D}_n = \frac{1}{\lambda_n} \langle (\mathbf{x} - \hat{\mathbf{x}}) r_n \rangle, \quad (\text{S.11})$$

and illustrates that the decoder will generally align with the direction of the largest reconstruction errors whenever the neuron fires strongly. An explicit solution can be found as well, corresponding to a penalized least square solution, and is given by

$$\mathbf{D} = \langle \mathbf{x} \mathbf{r}^\top \rangle \langle \mathbf{r} \mathbf{r}^\top + \mathbf{\Lambda} \rangle^{-1}.$$

where  $\mathbf{\Lambda}$  is a diagonal matrix whose entries are the Lagrangian constraints,  $\lambda_n$ .

## 1.7 The connectivity and thresholds of the optimal network

The optimal decoder allows us to find the best possible reconstruction for a given network. We emphasize that the ‘best possible reconstruction’ is not necessarily a good one; depending on the network connectivity, the reconstruction may not work at all. To counter this problem, we will study how to choose the free internal parameters of the network—the synaptic weights and the thresholds—such that the loss function is minimized. In other words, instead of assuming that the network is given, and then optimizing the decoder  $\mathbf{D}$ , we will now assume that the decoder is given, and we will then optimize the network. We will do so following the derivations layed out in [1].

First, we assume that we have a given and fixed decoder,  $\mathbf{D}$ . We can then consider the effect of a spike of neuron  $n$  on the loss  $\ell$  (S.10). The spike will increase the filtered spike train,  $r_n \rightarrow r_n + 1$ , and thus update the signal estimate according to  $\hat{\mathbf{x}} \rightarrow \hat{\mathbf{x}} + \mathbf{D}_n$ , where  $\mathbf{D}_n$  is the  $n$ -th column of the decoder matrix  $\mathbf{D}$ . We can therefore rewrite the objective (S.10) after the firing of the spike as

$$\ell(\text{neuron } n \text{ spiked}) = \|\mathbf{x} - \hat{\mathbf{x}} - \mathbf{D}_n\|^2 + \mu \|\mathbf{r} + \mathbf{e}_n\|^2 + \nu \|\mathbf{r} + \mathbf{e}_n\|_1,$$

where  $[\mathbf{e}_n]_j = \delta_{nj}$ . We adopt a greedy optimization scheme in which a neuron fires as soon as its spike decreases the loss. Mathematically, this condition yields the expression  $\ell(n \text{ spiked}) < \ell(n \text{ did not spike})$ , from which we can immediately derive the spiking condition [2, 1],

$$\mathbf{D}_n^\top \mathbf{x} - \mathbf{D}_n^\top \mathbf{D} \mathbf{r} - \mu r_n > \frac{1}{2} (\|\mathbf{D}_n\|_2^2 + \mu + \nu).$$

Notice that all terms on the l.h.s. are time-dependent while all terms on the r.h.s. are constant. We will identify the l.h.s. with the (time-varying) voltages of our neurons, and the r.h.s. with the (constant) thresholds,

$$V_n(t) = \mathbf{D}_n^\top \mathbf{x} - \mathbf{D}_n^\top \mathbf{D} \mathbf{r} - \mu r_n, \quad (\text{S.12})$$

$$T_n = \frac{1}{2} (\|\mathbf{D}_n\|_2^2 + \mu + \nu). \quad (\text{S.13})$$

In turn, if we take the temporal derivative of  $V_n$ , we obtain

$$\begin{aligned}\dot{V}_n &= \mathbf{D}_n^\top \dot{\mathbf{x}} - \mathbf{D}_n^\top \mathbf{D} \dot{\mathbf{r}} - \mu \dot{r}_n, \\ &= \mathbf{D}_n^\top (-\lambda \mathbf{x} + \mathbf{c}) - \mathbf{D}_n^\top \mathbf{D} (-\lambda \mathbf{r} + \mathbf{o}) - \mu (-\lambda r_n + o_n), \\ &= -\lambda V_n + \mathbf{D}_n^\top \mathbf{c} - (\mathbf{D}^\top \mathbf{D}_n + \mu \mathbf{e}_n)^\top \mathbf{o},\end{aligned}$$

where we used (S.1) and (S.2) in the second line, and (S.12) in the third line.

We have thereby derived a differential equation for the membrane voltage that can be compared with the equation for the general network of integrate-and-fire neurons, (S.5). To be optimal, a network should therefore have the following connectivity,

$$\begin{aligned}\mathbf{F} &= \mathbf{D}^\top, \\ \mathbf{\Omega} &= -\mathbf{D}^\top \mathbf{D} - \mu \mathbf{I} \\ &= -\mathbf{F} \mathbf{F}^\top - \mu \mathbf{I},\end{aligned}$$

where  $\mathbf{I}_N$  is the  $N \times N$  identity matrix.<sup>6</sup> These connectivities are similar to those of optimal rate networks that are designed to minimize the loss function (S.10) [3, 4, 5, 6]. They are quite specific in that the recurrent weights are symmetric and, as shown in the last equation, are directly related to the feedforward weights. Furthermore, the thresholds are similarly related to the recurrent (and thereby the feedforward connectivities) via (S.13) so that

$$\begin{aligned}\mathbf{T} &= \frac{1}{2} \left( \text{diag}(\mathbf{D}^\top \mathbf{D}) + \mu + \nu \right) \\ &= \frac{1}{2} \left( -\text{diag}(\mathbf{\Omega}) + \nu \right),\end{aligned}$$

where  $\mathbf{T}$  is simply the  $N$ -dimensional vector of all thresholds.

An important observation is that the spiking condition of a single neuron relies on local information only and does not require the evaluation or knowledge of the full objective function. Indeed, rewriting (S.12) by using the definition of  $\hat{\mathbf{x}}$ , we obtain

$$V_n(t) = \mathbf{D}_n^\top (\mathbf{x} - \hat{\mathbf{x}}) - \mu r_n, \quad (\text{S.14})$$

so that the voltage reflects both the part of the reconstruction error,  $\mathbf{x} - \hat{\mathbf{x}}$ , that is projected onto the decoder weights  $\mathbf{D}_n$ , as well as the quadratic cost term. Accordingly, a spike fired by a neuron is designed to decrease this projected error, and in turn decreases the objective [1].

## 1.8 The cost-term revisited

With the structure of the optimal network in mind, we can reconsider the importance of the cost term,  $C(\mathbf{r})$ . To do so, we imagine that there are (many) more neurons than independent inputs, i.e.,  $N > I$ . Ignoring spikes for a moment, and assuming graded firing rates  $\mathbf{r}$  and constant inputs  $\mathbf{x}$ , we observe that

---

<sup>6</sup>Note that, since we are now ignoring Dale's law, all synaptic weights can be both excitatory and inhibitory. For pedagogical purposes, however, it is often useful to consider the case in which all feedforward weights are excitatory, and hence all lateral weights are inhibitory (in the optimal network). We will make use of this toy case throughout the SI.

the solution space of (S.8) is degenerate in that many possible combinations of firing rates can minimize the objective. Possible solutions are those in which only a few neurons fire with high rates (sparse regime), and those in which many neurons fire with fairly low firing rates (dense regime).

The cost term allows us to control which solution the network converges to. The typical choice to enforce sparse population responses is a so-called *L1-cost*,  $C(\mathbf{r}) = \|\mathbf{r}\|_1 = \sum_n |r_n|$ , and the typical choice to enforce a dense population code is a so-called *L2-cost*  $C(\mathbf{r}) = \|\mathbf{r}\|_2^2 = \sum_n r_n^2$ . Many other costs such as slowness, group sparsity and others have been extensively discussed in the literature, especially in the context of regularization. We here adopt a linear sum of L1- and L2-cost for the rest of this manuscript, but the generalisation to other cost functions is possible with typically few modifications (see also [1] for a more detailed discussion).

## 2 The learning problem

Learning in recurrent neural networks can have different connotations. To clarify why we consider it a difficult problem, we will first review classical approaches and then describe exactly which problem we are trying to tackle.

### 2.1 Classical approaches to learning in recurrent neural networks

In ‘*top-down*’ approaches, one first specifies an objective that quantifies a network’s performance in a particular task, and then derives learning rules that modify the connectivity of the network to improve task performance. While this approach has mostly been used in *feedforward* neural networks, several approaches exist for *recurrent* neural networks. Famous examples include the Hebbian rules for Hopfield networks [7, 8], ‘backpropagation in time’ [9], or the more recent ‘FORCE’ learning algorithm [10].

The key problem with top-down approaches is that they often achieve their functionality at the cost of biological plausibility. First, almost all top-down approaches are based on ‘firing rate’ networks, i.e., networks in which neurons communicate with continuous rates rather than spikes. Second, most top-down approaches lead to ‘learning rules’ that are non-local, i.e., that depend on non-local information, such as the activity or synaptic weights of other neurons in the network.<sup>7</sup>

In ‘*bottom-up*’ approaches, the word ‘learning’ refers to networks whose synapses undergo specific, biologically plausible plasticity rules. In contrast to top-down approaches, the bottom-up perspective has allowed researchers to specifically investigate the effect of spike-timing-dependent plasticity on the dynamics of spiking networks. For instance, such rules may allow a network to learn how to properly balance itself on a specified time scale [11, 14].

The key problem with bottom-up approaches is that the generation of a particular dynamical regime does not necessarily imply any specific functionality. Indeed, bottom-up approaches usually run into problems when trying to

---

<sup>7</sup>The Hebbian rule for Hopfield networks is a famous exception to this case.

tie synaptic plasticity to computational goals. While several studies have delineated rules of thumb for how plausible learning rules may give rise to certain functions [15], they lack the insight or the mathematical guarantees that come with top-down approaches.

The difficulty of learning in recurrent neural networks is manifest in the gap between these two approaches: top-down approaches achieve functionality by sacrificing biological realism, and bottom-up approaches achieve biological realism by sacrificing functionality. A crucial challenge in bridging this gap turns out to be the locality constraint: biological synapses can only rely on local information in order to modify their strength. Indeed, deriving learning rules from an objective function under this locality constraint is often analytically intractable, and a large literature is devoted to this problem (distributed optimization; game theory; etc.). Most attempts at deriving local learning rules from functional principles have tried to circumvent this issue by approximating derived learning rules with local ones (e.g. [2, 5]). However, these approaches tend to work only under certain conditions and carry few mathematical guarantees in terms of optimality or convergence [16].

## 2.2 The efficient coding objective

Here our goal will be to bridge the gap and derive biologically realistic, local learning rules for a spiking network, that are guaranteed to converge to a specific global optimum. We will do this for the ‘autoencoder’, an unsupervised learning system that receives a set of time-varying input signals, and then learns to generate an efficient spike code in order to represent these signals. Given that our work is based on minimizing quadratic loss functions with linear and quadratic costs, algorithms such as principal component analysis (PCA) and independent component analysis (ICA) are special cases of this class of learning problems [17].

We will start by defining the objective of our network. In Section 1.7, we assumed a *given and fixed* decoder  $\mathbf{D}$ , and then derived a network that minimizes the objective <sup>8</sup>

$$L^* = \min_{\mathbf{o}} \left\langle \|\mathbf{x} - \mathbf{D}\mathbf{r}\|^2 + \mu \|\mathbf{r}\|^2 + \nu \|\mathbf{r}\|_1 \right\rangle.$$

Unfortunately, this objective cannot be used for learning a network, since the pre-defined decoder  $\mathbf{D}$  is not part of the network structure, and there is a priori no way the network can guess it.<sup>9</sup> Indeed, learning has to start in a network with random initial feedforward weights  $\mathbf{F}$  and recurrent weights  $\mathbf{\Omega}$ .

We therefore need to make a small change in perspective: instead of fixing a decoder upfront we require the network to perform a double-minimization with respect to both the spike times  $\mathbf{o}$  as well as with respect to the decoder  $\mathbf{D}$ ,

$$L^* = \min_{\mathbf{o}, \mathbf{D}} \left\langle \|\mathbf{x} - \mathbf{D}\mathbf{r}\|^2 + \mu \|\mathbf{r}\|^2 + \nu \|\mathbf{r}\|_1 \right\rangle \text{ s.t. } \|\mathbf{D}_n\|_2^2 = 2T_n - \mu - \nu, \quad (\text{S.15})$$

where the constraint on the decoder length arises from (S.13).

<sup>8</sup>Strictly speaking, the spike trains  $\mathbf{o}$  are obtained through a greedy minimization of the time-dependent loss  $\ell(t)$ . In practice, however, this approximation works quite well [1]

<sup>9</sup>Note that this decoder might even be chosen very badly and result in pathological cases such as one neuron firing with extremely high rates.

### 2.3 The problem of learning the synaptic weights

The objective function (S.15) seems to pose a baffling problem to solve with a neural network for multiple reasons: first, at the beginning of learning the decoder is not explicitly represented in the network connectivity, so how could the network ‘learn’ a decoder? Second, neither the feedforward nor the recurrent weights are explicitly part of the objective, (S.15). Rather, the instantaneous firing rates,  $\mathbf{r}(t)$ , depend implicitly on the connectivity. Hence, even a simple gradient descent with respect to the synaptic weights is not possible. Third, even if the feedforward weights are initially set to the correct values, i.e., to the values of the optimal decoder  $\mathbf{D}^*$ , i.e.  $\mathbf{F} = \mathbf{D}^{*\top}$ , we could still not learn the desired recurrent connectivity  $\mathbf{\Omega} = -\mathbf{F}\mathbf{F}^\top - \mu\mathbf{I}$ . The key problem is that neurons have no direct access to their respective feedforward weights. More precisely, the input to the network is given by  $\mathbf{F}\mathbf{x}$ , but from the perspective of the network  $\mathbf{F}$  and  $\mathbf{x}$  are only defined up to a linear orthogonal transformation  $\mathbf{A}$ ,  $\mathbf{F}\mathbf{x} = (\mathbf{F}\mathbf{A}^\top)(\mathbf{A}\mathbf{x})$ . Before showing how we can address these problems, we will briefly discuss a fourth issue, concerning the thresholds  $T_n$  of the neurons and their relation to the length of the decoder.

### 2.4 The problem of the appropriate decoder scale

Section 1.7 showed that the thresholds,  $T_n$  are intimately linked to the length of the decoder weights. To address this problem, we introduced a constraint on the length of the decoders in the double-minimization (S.15). In practice, we will therefore assume that the thresholds,  $T_n$ , are constant throughout learning and then re-interpret (S.13) as imposing a constraint on the length of the decoder weights,

$$\|\mathbf{D}_n\|_2^2 = 2T_n - \mu - \nu.$$

In turn, this ‘scaling constraint’ effects the scaling of both the feedforward and recurrent weights. Using our knowledge of the optimal architecture,  $\mathbf{F}^\top = \mathbf{D}$  and  $\mathbf{\Omega} = -\mathbf{D}^\top\mathbf{D} - \mu\mathbf{I}$ , we can directly interpret the constraint on the decoder as constraints on the feedforward and recurrent connectivity, namely

$$\begin{aligned}\|\mathbf{F}_n\|_2^2 &= 2T_n - \mu - \nu, \\ -\Omega_{nn} &= \|\mathbf{D}_n\|_2^2 + \mu = 2T_n - \nu.\end{aligned}$$

These scaling constraints need to be taken into account when learning the synaptic connectivity. However, it is important to note that the constraints only change the scale but not the structure of the network connectivity. For this reason, and in order to concentrate on the core intuitions behind the learning rule, we will delay the treatment of the scaling problem until section 4.7.

## 3 The core intuitions behind learning

The last section showed that we need to exploit some other property of the network in order to be able to learn the desired connectivity. In this section, we will explain the core intuitions behind our learning rules and show why the balance between excitation and inhibition is tied to the quality of the output code and to the desired network architecture. While this section does not consider

the most general scenario (with both L1 and L2 costs and correct scaling), we will revisit this issue in section 4, where the actual learning rules used in the main paper are derived. In order to simplify things, we will first neglect the cost terms  $\mu$  and  $\nu$ .

### 3.1 Error-driven coding

The ‘locality of information’ constraint suggests that the learning problem should be attacked from the point of view of the single neuron. The membrane voltage of one of our neurons will initially obey (S.6), which we here re-express for the  $n$ -th neuron,

$$V_n = \mathbf{F}_n^\top \mathbf{x} + \mathbf{\Omega}_n^\top \mathbf{r},$$

where the first term is the feedforward input and the second term the recurrent input.

To understand what our neuron should do with its synapses, we will first consider what happens at the level of this neuron, once the input signal can be properly reconstructed from the network output with some decoder  $\mathbf{D}$ . We emphasize that we do not assume that we know the shape of  $\mathbf{D}$  or that we are already in the optimal architecture (Section 1.7). Rather, we will simply assume that the network is in *some* state in which *some* decoder  $\mathbf{D}$  will properly do the job, in which case the reconstruction error should be very small, so that  $\mathbf{x} - \hat{\mathbf{x}} \approx 0$ .

From the point of view of the  $n$ -th neuron, this reconstruction error is inaccessible. Indeed, our neuron only receives a small part of the input signal, namely the input signal as seen through the lense of its feedforward weights,  $\mathbf{F}_n^\top \mathbf{x}$ . However, the reconstruction error  $\varepsilon_n$  for this part of the input signal should, of course, likewise be close to zero so that

$$\begin{aligned} \varepsilon_n &= \mathbf{F}_n^\top \mathbf{x} - \mathbf{F}_n^\top \hat{\mathbf{x}} \\ &= \mathbf{F}_n^\top \mathbf{x} - \mathbf{F}_n^\top \mathbf{D} \mathbf{r} \\ &\approx 0. \end{aligned}$$

Our key insight is now that this latter equation will be identical to the voltage equation if we assume that  $\mathbf{\Omega}_n^\top = -\mathbf{F}_n^\top \mathbf{D}$  and  $\varepsilon_n = V_n \approx 0$ . Hence, we have obtained two *sufficient* conditions for the network to properly represent the input signals. If we can furthermore ensure that the feedforward weights align with the decoder, and that  $\mathbf{D} = \mathbf{D}^*$ , then we have learnt the optimal architecture from Section 1.7, and found the minimum of the loss function (S.15).

### 3.2 The four conditions of learning

These insights lead us to the following *four conditions* of learning:

1. The membrane voltage of each neuron should remain close to zero, i.e., its resting potential. We can interpret this to mean that the membrane voltage fluctuations should be minimized or bounded as tightly as possible. Accordingly, any deviation from rest caused by the feedforward inputs must be immediately eliminated by the recurrent inputs. In other words, the feedforward and recurrent inputs into each cell need to balance each other on short time-scales. As a consequence, any excitatory input into

the cells must be quickly canceled by an inhibitory input of equal size, a condition known as E/I balance.

2. The recurrent connectivity should be of the form  $\mathbf{\Omega} = -\mathbf{FD}$  where  $\mathbf{D}$  is an a priori unknown decoder matrix. As a consequence, the membrane voltage of each neuron can be interpreted as a *projection of the reconstruction error*,  $\varepsilon_n$ , which we will refer to as ‘error-driven coding.’ Indeed, the recovery of the reconstruction error in the membrane voltages is a key ingredient of the optimal network, see equation (S.14). We emphasize that the decoder matrix,  $\mathbf{D}$ , is unspecified at this point, and that not all matrices  $\mathbf{D}$  will allow a network to fulfill condition (1), as well. As a consequence, the target  $\mathbf{\Omega} = -\mathbf{FD}$  consists of a large, if unspecified, set of possible matrices, and ‘error-driven coding’ can be achieved by a large set of networks.
3. The network architecture that we have derived so far deviates from the optimal architecture, since  $\mathbf{F}$  and  $\mathbf{D}^\top$  are not necessarily the same matrices. Accordingly, we need to somehow make sure that the feedforward weights  $\mathbf{F}$  align with the (unknown) decoder  $\mathbf{D}^\top$ .
4. All of these conditions take the point of view of the single neuron. To make sure that the network as a whole represents the input signals properly, the feedforward weights need to properly span the space of input signals. If, for instance, the feedforward weights of all neurons were identical, the network could at most represent the one-dimensional space spanned by these feedforward weights. This condition will be automatically fulfilled if both  $\mathbf{D}$  and  $\mathbf{F}$  converge to the global optimum  $\mathbf{D}^*$  of (S.15).

These conditions suggest a specific program for learning the synaptic weights. First, starting from random feedforward and recurrent weights, we need to learn a balanced system in which the recurrent weights converge to a low-rank solution,  $\mathbf{\Omega} \rightarrow -\mathbf{FD}$ . In a second step, we can then aim to tighten the balance between excitatory and inhibitory currents by aligning  $\mathbf{D}$  and  $\mathbf{F}$  such that both converge to the global optimum,  $\mathbf{D}^*$ .<sup>10</sup>

In the following two subsections we derive a local learning rule for the recurrent synapses for which the fixed points obey properties (1) and (2). For an even tighter balance, we then introduce a learning mechanism for the feedforward synapses that will make the network structure converge to the solution (S.12) of the quadratic optimization problem (S.15).

### 3.3 Condition 1: Recurrent weights learn to balance feedforward inputs spike by spike

The shortest possible time-scale at which a single spiking neuron can be balanced is limited by the interval between any two consecutive spikes of the *population*. We will refer to this interval as a population interspike interval (pISI), in contrast to the standard interspike interval (ISI) that is defined for two consecutive spikes of the *same* neuron.

---

<sup>10</sup>We re-emphasize that the decoder  $\mathbf{D}$  is *not* a biophysical quantity of the network. However, it does serve as an important *conceptual* tool that is central to the development of the learning rules.

We illustrate this idea in Figure 1D in the main text. Here a cell receives excitatory feedforward inputs and inhibitory spikes from three pre-synaptic neurons. Between the second and the third spike (gray area) the cell integrates its feedforward input currents and depolarizes its membrane voltage. The arrival of the second inhibitory spike (red) then causes a hyperpolarization of the membrane potential (see voltage trace in middle panels). In the balanced case (left column) the hyperpolarization due to the inhibitory spike from the red neuron perfectly cancels the depolarization through the excitatory feedforward connections (gray area).

To understand how to balance a single cell on such a short time-scale, we rewrite the membrane potential as a sum over spikes. We index the spikes in the network by the time of their occurrence, writing  $t_1, t_2, \dots$  for the successive spike times of the population. We then introduce a second index in order to identify which neuron fired a particular spike, writing  $k(i)$  to indicate that the  $i$ -th spike,  $t_i$ , was fired by the  $k$ -th neuron. With this notation in mind, let us define the integral over the input signal  $\mathbf{c}(t)$  in the interval between two consecutive population spikes at time  $t_{i-1}$  and  $t_i$ :

$$\mathbf{g}(t_i) := \int_{t_{i-1}}^{t_i} d\tau \mathbf{c}(\tau) e^{-\lambda(t_i - \tau)}.$$

We can then write the membrane voltage  $V_n(t_i)$  at time  $t_i$  (i.e. at the time of the  $i$ -th spike) as (confer (S.6))

$$\begin{aligned} V_n(t_i) &= \mathbf{F}_n^\top \mathbf{x} + \mathbf{\Omega}_n^\top \mathbf{r} \\ &= \mathbf{F}_n^\top \int_0^\infty d\tau \mathbf{c}(\tau) e^{-\lambda(t_i - \tau)} + \mathbf{\Omega}_n^\top \int_0^\infty d\tau \mathbf{o}(\tau) e^{-\lambda(t_i - \tau)} \\ &= \sum_{j \leq i} \mathbf{F}_n^\top \mathbf{g}(t_j) e^{-\lambda(t_i - t_j)} + \sum_{j \leq i} \mathbf{\Omega}_{nk(j)} e^{-\lambda(t_i - t_j)} \\ &= \sum_{i \leq j} (\mathbf{F}_n^\top \mathbf{g}(t_j) + \mathbf{\Omega}_{nk(j)}) e^{-\lambda(t_i - t_j)}, \end{aligned}$$

where  $k(j)$  denotes the index of the neuron spiking at time  $t_j$ , as explained above. Here  $\mathbf{F}_n \mathbf{g}(t_j)$  corresponds to the accumulated excitatory current during the pISI before the  $j$ -th spike, i.e., the total charge transfer. In turn,  $\mathbf{\Omega}_{nk(j)}$  corresponds to the immediate inhibitory charge transfer caused by the  $j$ -th spike itself. The network is perfectly balanced on the shortest time scale if these two opposing charge transfers cancel exactly. In more practical terms, the network is balanced on the shortest time scale if the (squared) net charge transfer,  $(\mathbf{F}_n^\top \mathbf{g}(t_j) + \mathbf{\Omega}_{nk(j)})^2$ , is as small as possible.

We hence concentrate on minimizing the objective

$$L = \sum_{n,i} \left( \mathbf{F}_n^\top \mathbf{g}(t_i) + \mathbf{\Omega}_{nk(i)} \right)^2,$$

where the sum runs over both neurons,  $n$ , and spike times,  $i$ . We can minimize this objective by updating the recurrent synaptic weights after each spike in a

greedy manner,

$$\Delta\Omega_{nk}(t) \propto \begin{cases} -\mathbf{F}_n^\top \mathbf{g}(t) - \Omega_{nk}(t) & \text{when neuron } k \text{ spikes,} \\ 0 & \text{otherwise.} \end{cases} \quad (\text{S.20})$$

This rule has a rather intuitive meaning, as explained in the main paper and illustrated in Fig 1D: if the excitation a neuron receives in the last pISI is higher than the subsequent lateral inhibition, inhibition is strengthened, and vice versa<sup>11</sup>. Importantly, the learning rule relies only on local information, i.e. on quantities that are available to the neuron that needs to update its synapses.

### 3.4 Condition 2: Spike-by-spike balance results in error-driven coding

By using the above learning rule for the recurrent weights, we can establish spike-by-spike balance—condition (1) in Section 3.1—for every single neuron  $n = 1 \dots N$ . We will now show that error-driven coding—condition (2)—comes out as a by-product of this learning rule.

The proof is straightforward. We simply investigate the fixed points of the learning rule (S.20), i.e. all points for which the mean update is zero,  $\langle \Delta\Omega \rangle = 0$ . We obtain

$$\Omega_{nk} = -\left\langle \mathbf{F}_n^\top \mathbf{g} \right\rangle_{k \text{ spikes}} = -\mathbf{F}_n^\top \langle \mathbf{g} \rangle_{k \text{ spikes}},$$

where the brackets denote an average taken over all the spike-times of neuron  $k$ . This formula has two interesting consequences. First, the strength of the inhibitory synapse from neuron  $k$  to neuron  $n$  equals the average excitatory feedforward current that neuron  $n$  receives in the pISI before a spike of neuron  $k$ . Thus, all neurons in the population cooperate to keep the voltage of the post-synaptic cell as constant as possible. Second, the fixed points for the recurrent weights can be written as  $\Omega_{nk} = -\mathbf{F}_n^\top \mathbf{D}_k$  where<sup>12</sup>

$$\mathbf{D}_k = \langle \mathbf{g} \rangle_{k \text{ spikes}}. \quad (\text{S.21})$$

We note that this is the desired low-rank factorization for “error-driven coding”, i.e.,  $\Omega \rightarrow -\mathbf{F}\mathbf{D}$ . In this regime the membrane voltage of each cell tracks a projection of the error, and so the network fulfills condition (2) in section 3.1.

To summarize, we derived a simple learning rule for the recurrent connections from the principle that each recurrently fired spike should balance the feedforward input of its respective postsynaptic cells. This rule seeks to balance the network on the shortest possible time scale and thereby yields the desired low-rank factorization of the recurrent weights which is important for error-driven coding. Furthermore, we have derived an explicit formula for the decoder. Hence, even though the decoder was initially unknown, and even though the decoder does not have a direct biophysical manifestation, it can be computed through biophysical quantities, namely, the input signal sampled at the spikes of the different neurons.

<sup>11</sup>Note once more that, for illustrative purposes, we here suppose that the recurrent weights are inhibitory and all feedforward weights are excitatory. We use this simplified picture for the rest of the SI. In the case described here, in which the network violates Dale’s law, feedforward and recurrent weights can have both positive as well as negative signs.

<sup>12</sup>Please note that  $\mathbf{F}_k$  corresponds to the  $k$ -th *row* of matrix  $\mathbf{F}$  while  $\mathbf{D}_k$  corresponds to the  $k$ -th *column* of matrix  $\mathbf{D}$ . Nonetheless, all vectors in the SI, including these two, are assumed to be column vectors.

### 3.5 Interlude: The importance of quadratic costs

The ‘error-driven coding’ architecture,  $\mathbf{\Omega} = -\mathbf{FD}$ , achieves the primary objective, i.e. representing the signal  $\mathbf{x}(t)$ , which can now be read out via the decoder  $\mathbf{D}$ . The efficiency of the representation, however, depends on the exact choice of the feedforward weights. More specifically, there are two problems. First, if the feedforward weights do not cover some part of the input space (as in Figure 2, left column), then the reconstruction cost can still be high in that part of the space. Second, even if the feedforward weights cover the whole space, so that  $\hat{\mathbf{x}} \approx \mathbf{x}$  everywhere, the particular spiking code chosen by the system can still be wildly inefficient: since we have not considered any cost terms, neurons could fire at very high rates in order to properly represent the signal. To find a better distribution of the feedforward weights, we therefore need to first reintroduce the L2 cost term, i.e., the cost term that severely punishes high firing of individual neurons.

In the presence of an L2 cost, we know the form of the optimal recurrent connectivity from section 1.7. Adapted to the error-driven coding architecture, the recurrent weights should therefore converge to  $\mathbf{\Omega} = -\mathbf{FD} - \mu\mathbf{I}$ . We can achieve this new fixed point of the recurrent learning rule (S.20) by introducing a small regularization term,  $\mu\delta_{ij}$ , so that

$$\Delta\Omega_{nk}(t) \propto \begin{cases} -\mathbf{F}_n^\top \mathbf{g}(t) - \Omega_{nk}(t) - \mu\delta_{nk} & \text{when neuron } k \text{ spikes,} \\ 0 & \text{otherwise.} \end{cases} \quad (\text{S.22})$$

Importantly, the learning rule will still seek to balance the system as tightly as possible given the extra constraints. Following the logic of the previous section, one can see that  $\mathbf{\Omega}$  will converge to the desired fixed point. After convergence of the recurrent weights to  $\mathbf{\Omega} = -\mathbf{FD} - \mu\mathbf{I}$ , the membrane potential of each neuron can be written as

$$\mathbf{V} = \mathbf{F}(\mathbf{x} - \mathbf{D}\mathbf{r}) - \mu\mathbf{r}.$$

As a side note, we point out that the introduction of the cost term does not alter the definition of the decoder (S.21).

### 3.6 Condition 3: Feedforward weights learn to mimic the decoder

The derivation of the optimal network, section 1.7, suggests that  $\mathbf{F}$  should eventually align with  $\mathbf{D}^\top$ , as explained in condition (3) in section 3.1. Ideally, one would therefore want an update rule of the form  $\Delta\mathbf{F} \propto \mathbf{D}^\top - \mathbf{F}$ , which would move the feedforward weights towards the decoder  $\mathbf{D}^\top$ . Unfortunately, this learning rule is not biophysically realistic since  $\mathbf{D}$  is not an explicit quantity in the network. However, using the fixed-point equation for the decoder, (S.21), we can replace  $\mathbf{D}$  to obtain a local, biophysical rule

$$\Delta\mathbf{F}_n(t) \propto \begin{cases} \mathbf{g}(t) - \mathbf{F}_n(t) & \text{when neuron } k \text{ spikes,} \\ 0 & \text{otherwise.} \end{cases}$$

If the learning of the feedforward connectivity occurs more slowly than the learning of the recurrent connectivity, then all fixed points of the feedforward

network connectivity will fulfill  $\mathbf{F}_n = \langle \mathbf{g} \rangle_{n \text{ spikes}} = \mathbf{D}_n$  and hence  $\mathbf{F} \rightarrow \mathbf{D}^\top$  as desired. From a biophysical perspective the first term in the learning rule,  $\langle \mathbf{g} \rangle_{n \text{ spikes}}$ , corresponds to the average input signal integrated before a spike of neuron  $n$ . Such a signal could be computed in the presynaptic terminal, for instance, which, given the complex machinery of synaptic plasticity is well within the realm of possibilities.

We make two observations about the feedforward rule. First, the rule will only change the feedforward weights if a postsynaptic spike (of neuron  $n$ ) coincides with a previous presynaptic input (the integrated input signal up to the time of the postsynaptic spike). In other words, this learning rule corresponds to the causal part of the standard STDP-rule (see Figure 3Ai in the main text). Second, a neuron that never spikes will not change its feedforward weight. We do not consider this scenario here, but simply note that it can be prevented by introducing a noise term in the learning rule.

### 3.7 Condition 4: Learning rules minimize loss function

While the feedforward learning rule shapes the connectivity into the desired form (section 1.7), it is not a priori clear whether these changes also help to minimize the loss function, (S.15), which was our fourth condition on learning. We will now show that the learning rule derived in the previous section achieves exactly that. To do so, we will investigate how the learning rules affect the (average) voltages, since the voltages are directly linked to the reconstruction errors and thereby the loss function. To keep things simple, we will assume that the recurrent connectivity is already learnt, and we will write  $\Delta \mathbf{F} \propto \mathbf{D}^\top - \mathbf{F}$  for the feedforward update. The resulting change in the voltage will then—on average—be proportional to

$$\begin{aligned} \Delta \mathbf{V} &= \langle \Delta \mathbf{F}(\mathbf{x} - \mathbf{D}\mathbf{r}) \rangle, \\ &\propto \langle (\mathbf{D}^\top - \mathbf{F})(\mathbf{x} - \mathbf{D}\mathbf{r}) \rangle, \\ &= \langle \mathbf{D}^\top(\mathbf{x} - \mathbf{D}\mathbf{r}) - \mu\mathbf{r} \rangle - \langle \mathbf{F}(\mathbf{x} - \mathbf{D}\mathbf{r}) - \mu\mathbf{r} \rangle \\ &= \langle \mathbf{D}^\top(\mathbf{x} - \mathbf{D}\mathbf{r}) - \mu\mathbf{r} \rangle - \langle \mathbf{V} \rangle. \end{aligned}$$

Since the learning of  $\mathbf{F}$  happens on a much slower time-scale than the learning of the recurrent weights, the second term on the r.h.s., i.e., the average voltage, will be close to zero, as the network remains in a tightly balanced state throughout the learning of the feedforward weights. Accordingly, the first term will dominate changes in the voltage so that

$$\begin{aligned} \Delta \mathbf{V} &\propto \langle \mathbf{D}^\top(\mathbf{x} - \mathbf{D}\mathbf{r}) - \mu\mathbf{r} \rangle, \\ &\propto -\frac{\partial L}{\partial \mathbf{r}} \end{aligned}$$

where  $L$  is the averaged loss function (S.8) in the absence of the linear cost term. In other words, the change in voltage will push the instantaneous firing rate of the network in the direction of the antigradient of the loss function, thus minimising it.

### 3.8 Conclusions and biological realism reconsidered

To summarize, in this section we illustrated how an STDP-like learning rule for the feedforward connections in conjunction with a recurrent learning rule that seeks to tightly balance excitatory and inhibitory inputs, leads to a network architecture that optimizes the average loss, (S.8), and thereby produces an efficient spike code of the input signals. The derived learning rules are local, in that they only require knowledge of quantities that are available to the neurons.

There are several issues that we did not consider so far. First, we did not study linear costs or non-whitened input distributions. Second, even though the learning rules are local, their biological plausibility may still be questioned, since the rules require the integration of input currents between successive spikes of the population. While it cannot be ruled out that actual neurons (or synapses) do keep track of these quantities, it has not been observed, either. In the next section, we address these concerns and derive learning rules based on the voltages of the neurons. We furthermore consider the extension to linear costs, non-whitened inputs, correct scaling and, finally, the full E/I network.

## 4 The Voltage-based learning rules

In this section, we will derive the learning rules described in the main text. The derivation in this section follows the spirit of the last section. To recapitulate, in order to improve the ability of our network to properly encode the input signals, we need to satisfy four conditions. First, the recurrent weights of each neuron need to learn to balance the feedforward inputs spike by spike. Second, the recurrent connectivity needs to converge to  $\mathbf{\Omega} \rightarrow -\mathbf{FD} - \mu\mathbf{I}$  for a suitable decoder  $\mathbf{D}$ . Third, the membrane fluctuations need to be further tightened moving the feedforward weights to  $\mathbf{F} \rightarrow \mathbf{D}^\top$ , and the recurrent weights to  $\mathbf{\Omega} \rightarrow -\mathbf{D}^\top\mathbf{D} - \mu\mathbf{I}$ . Fourth, we need to make sure that the joint interaction of the learning rules minimizes our global loss function.

### 4.1 Recurrent weights: Learning in the absence of cost terms

As in section 3.4, we start by considering the learning of the recurrent synapses without costs. The target of learning is then a balanced network with recurrent weights  $\mathbf{\Omega} = -\mathbf{FD}$ . In the last section we showed that it is enough to seek a balanced state in order to reach both properties. In the same spirit, we first establish a suitable and practical measure of membrane voltage fluctuations, derive learning rules for the recurrent weights that minimize those fluctuations and then show that the network will converge to a low-rank configuration  $\mathbf{\Omega} \rightarrow -\mathbf{FD}$ .

A particularly straightforward way of measuring voltage fluctuations is the temporal average of the squared voltage deviations from rest  $V_0 = 0$ , i.e.,

$$L = \left\langle \|\mathbf{V}(t)\|^2 \right\rangle_t.$$

However, evaluating the exact voltage deviations requires a precise tracking of the membrane voltage at all times, and may thus be infeasible for real neurons. Inspired by the insights from the previous section, we start with the presumption

that learning occurs only during the presence of a presynaptic spike. We can then reduce the problem to minimizing the deviations of the membrane voltages around the time of a presynaptic spike. In the optimal network, the membrane voltage of a spiking neuron jumps from the threshold,  $T$ , *before* the spike to the reset,  $-T$ , *after* the spike. Similarly, to achieve tight balance the membrane voltage of all other neurons should ideally jump from  $+V$  before a presynaptic spike to  $-V$  after the spike. This motivates the following spike-based measure of the membrane voltage fluctuations,

$$L = \left\langle \left\| \frac{1}{2} \left( \mathbf{V}^{\text{before}}(t_j) + \mathbf{V}^{\text{after}}(t_j) \right) \right\|^2 \right\rangle_{\text{spikes}} \quad (\text{S.23})$$

where  $t_j$  is the time of the  $j$ -th spike in the population and  $\langle \cdot \rangle_{\text{spikes}}$  denotes the expectation value over those spikes<sup>13</sup>. The superscripts “before” and “after” refer to the voltage values immediately before and after a spike. The recurrent weights enter (S.23) through their effect on the post-spike membrane potential,

$$\mathbf{V}^{\text{after}}(t_j) = \mathbf{V}^{\text{before}}(t_j) + \mathbf{\Omega} \mathbf{e}_{k(j)},$$

where  $k(j)$  is again the index of the neuron that spikes at time  $t_j$  and  $\mathbf{e}_{k(j)}$  is a unit vector with zero entries except at position  $k(j)$ . The introduction of  $\mathbf{e}_{k(j)}$  is a bit cumbersome but useful: it allows, for example, to write the relation between the instantaneous rates of the whole population before and after a spike of neuron  $k$  at time  $t_j$  as a simple vector equation,

$$\mathbf{r}^{\text{after}}(t_j) = \mathbf{r}^{\text{before}}(t_j) + \mathbf{e}_{k(j)}.$$

The deviation at time  $t_j$  is thus

$$\begin{aligned} L_j &= \left\| \frac{1}{2} \left( \mathbf{V}^{\text{before}}(t_j) + \mathbf{V}^{\text{after}}(t_j) \right) \right\|^2 \\ &= \left\| \mathbf{V}^{\text{before}}(t_j) + \frac{1}{2} \mathbf{\Omega} \mathbf{e}_{k(j)} \right\|^2. \end{aligned}$$

To minimize the voltage deviations, we perform a greedy optimization every time a spike was fired by one of the neurons in the network,

$$\Delta \mathbf{\Omega}(t_j) \propto -\frac{\partial L_j}{\partial \mathbf{\Omega}} \propto -\left( 2\mathbf{V}^{\text{before}}(t_j) + \mathbf{\Omega} \mathbf{e}_{k(j)} \right) \mathbf{e}_{k(j)}^\top. \quad (\text{S.24})$$

More explicitly, the weight  $\Omega_{nk}$  is updated at every spike of the presynaptic neuron  $k = k(j)$  such that the deviation of the postsynaptic membrane voltage from rest is minimized,

$$\Delta \Omega_{nk}(t_j) \propto \begin{cases} -2V_n^{\text{before}}(t_j) - \Omega_{nk} & \text{if } k \text{ spiked,} \\ 0 & \text{otherwise.} \end{cases} \quad (\text{S.25})$$

This learning rule differs from the one in the last section mainly in the first term on the r.h.s.: instead of compensating for the integrated feedforward current during the last pISI, the synapses here learn to compensate for the deviation of the membrane voltage from rest.

<sup>13</sup>Note that in practice, i.e., in numerical simulations, we replace this expectation value with a moving sum over a sufficiently large number of spikes. More precisely, we replace  $\langle x \rangle_{\text{spikes}} = \frac{1}{J} \sum_{j=1}^J x(t_j)$  where  $t_j$  is the spike-time of the  $j$ -th spike in the past (relative to the current time  $t$ ).

## 4.2 Recurrent weights: Fixed point analysis

In this section we show that the fixed-points (i.e. the points at which the mean change in the recurrent weights is zero) of the learning rule (S.25) are of the desired low-rank configuration  $\mathbf{\Omega} \rightarrow -\mathbf{F}\mathbf{D}$ . In the next section we will then prove that the system will globally converge to one of these fixed-points under mild assumptions.

Mathematically, the fixed-points are defined as those recurrent weights for which  $\langle \Delta \mathbf{\Omega} \rangle_{\text{spikes}} = 0$ . All quantities below, such as  $\mathbf{V}(t_j)$ ,  $\mathbf{x}(t_j)$ , etc., are to be understood as immediately *before* a spike, and we hence drop the superscript “before” for the rest of the SI, as well as the explicit reference to the spike time,  $t_j$ , for ease of notation<sup>14</sup>. The learning rule, (S.24), can be rewritten as

$$\begin{aligned} \Delta \mathbf{\Omega} &\propto -2\mathbf{V}\mathbf{e}_{k(j)}^\top - \mathbf{\Omega}\mathbf{e}_{k(j)}\mathbf{e}_{k(j)}^\top \\ &\stackrel{\text{(S.6)}}{=} -2(\mathbf{F}\mathbf{x} + \mathbf{\Omega}\mathbf{r})\mathbf{e}_{k(j)}^\top - \mathbf{\Omega}\mathbf{e}_{k(j)}\mathbf{e}_{k(j)}^\top \\ &= -2\mathbf{F}\mathbf{x}\mathbf{e}_{k(j)}^\top - \mathbf{\Omega}(2\mathbf{r} + \mathbf{e}_{k(j)})\mathbf{e}_{k(j)}^\top. \end{aligned} \quad (\text{S.26})$$

To investigate the fixed points, we need to study the effect of applying this learning rule repeatedly, i.e., over many spike times  $t_j$ . From (S.26) and the fixed-point condition  $\langle \Delta \mathbf{\Omega} \rangle_{\text{spikes}} = 0$  we obtain the defining property of the fixed points of the recurrent weights,

$$2\mathbf{F} \left\langle \mathbf{x}\mathbf{e}_{k(j)}^\top \right\rangle_{\text{spikes}} = -\mathbf{\Omega} \left\langle (2\mathbf{r} + \mathbf{e}_{k(j)})\mathbf{e}_{k(j)}^\top \right\rangle_{\text{spikes}}.$$

Under the mild condition that the sum on the r.h.s. has full rank we can directly infer that any fixed point of  $\mathbf{\Omega}$  is of the form  $-\mathbf{F}\mathbf{D}$  where  $\mathbf{D}$  is defined by

$$2 \left\langle \mathbf{x}\mathbf{e}_{k(j)}^\top \right\rangle_{\text{spikes}} = \mathbf{D} \left\langle (2\mathbf{r} + \mathbf{e}_{k(j)})\mathbf{e}_{k(j)}^\top \right\rangle_{\text{spikes}}. \quad (\text{S.27})$$

While the matrix  $\mathbf{D}$  can be interpreted as a linear decoder, which one could use to reconstruct the input signal from the spike trains, it is not explicitly realized within the network, since it is merged into the recurrent weights and arises dynamically through learning. In other words, the decoder is not defined upfront but the recurrent connectivity converges to a low-rank factorization from which an external observer can read off the linear decoder.

Note that (S.27) is a matrix equation with dimensions  $I \times N$ . To understand the exact nature of the arising decoder  $\mathbf{D}$  it is instructive to look at each element  $i, n$  individually,

$$\begin{aligned} 2 \langle x_i \delta_{n,k(j)} \rangle_{\text{spikes}} &= \mathbf{D}_i^\top \langle (2\mathbf{r} + \mathbf{e}_{k(j)}) \delta_{n,k(j)} \rangle_{\text{spikes}}, \\ \Leftrightarrow 2 \langle x_i \rangle_{n \text{ spikes}} &= \mathbf{D}_i^\top \langle 2\mathbf{r} + \mathbf{e}_n \rangle_{n \text{ spikes}}, \end{aligned}$$

where  $\langle \cdot \rangle_{n \text{ spikes}}$  is simply an average over all the spikes of neuron  $n$ . Using the definition for the readout, (S.7), we obtain

$$\begin{aligned} \Leftrightarrow 2 \langle x_i \rangle_{n \text{ spikes}} &= 2 \langle \hat{x}_i \rangle_{n \text{ spikes}} + D_{in}, \\ \Leftrightarrow D_{in} &= 2 \langle x_i - \hat{x}_i \rangle_{n \text{ spikes}}. \end{aligned} \quad (\text{S.28})$$

<sup>14</sup>We note that the input signal  $\mathbf{x}(t_j)$  does not jump at the time  $t_j$  of the presynaptic spike, hence the distinction between before and after is irrelevant for this quantity.

Accordingly, the elements of the decoder are aligned with the reconstruction errors at the time of a spike. During learning, the optimal decoder will therefore move in directions with the largest error and hence will aim to cover as best as possible the signal space.<sup>15</sup>

The resulting relation for the decoder is essentially equivalent to the constraint optimal decoder derived in section 1.6, up to a scaling parameter, which we will consider further down. The minimum of the constraint loss function was found as (S.11)

$$D_{in}^* \propto \langle (x_i - \hat{x}_i) r_n \rangle_t .$$

Accordingly, the weighting of the error by the instantaneous firing rate mirrors the weighting of the error by the spikes in (S.28).

### 4.3 Recurrent weights: Convergence proof

In the last subsection we derived that all fixed points of the recurrent weights are of the form  $-\mathbf{F}\mathbf{D}$ , but these fixed points might be unstable. We here show that any spiking network with bounded membrane voltages will converge to the desired low-rank factorization.

To this end we split the recurrent weights  $\mathbf{\Omega}$  into a part that can be described by a low-rank factorization,  $\mathbf{\Omega}_F = -\mathbf{F}\mathbf{D}$  for some  $\mathbf{D}$ , and a residual part,  $\mathbf{\Omega}_\perp = \mathbf{\Omega} - \mathbf{\Omega}_F$ . In order to show that the recurrent weights  $\mathbf{\Omega}$  converge to  $\mathbf{\Omega}_F$ , we need to prove that the average update of  $\mathbf{\Omega}$  will always decrease the norm of the residual,  $\mathbf{\Omega}_\perp$ .

More precisely,  $\mathbf{\Omega}_F$  can be described as the projection of  $\mathbf{\Omega}$  onto the image of  $\mathbf{F}$ , i.e.  $\mathbf{\Omega}_F = \mathbf{F}\mathbf{F}^+ \mathbf{\Omega}$  where the superscript "+" denotes the Moore-Penrose pseudo-inverse. Vice versa, the residual is given by  $\mathbf{\Omega}_\perp = (\mathbf{I} - \mathbf{F}\mathbf{F}^+) \mathbf{\Omega}$  and so

$$\begin{aligned} \mathbf{\Omega} &= \mathbf{F}\mathbf{F}^+ \mathbf{\Omega} + (\mathbf{I} - \mathbf{F}\mathbf{F}^+) \mathbf{\Omega}, \\ &\equiv \mathbf{\Omega}_F + \mathbf{\Omega}_\perp. \end{aligned}$$

The update of  $\mathbf{\Omega}_\perp$  is the corresponding projection of the total update of the recurrent weights (S.26),

$$\begin{aligned} \Delta \mathbf{\Omega}_\perp &= (\mathbf{I} - \mathbf{F}\mathbf{F}^+) \Delta \mathbf{\Omega}, \\ &= (\mathbf{I} - \mathbf{F}\mathbf{F}^+) \left( -2\mathbf{F}\mathbf{x}\mathbf{e}_{k(j)}^\top - \mathbf{\Omega} (2\mathbf{r} + \mathbf{e}_{k(j)}) \mathbf{e}_{k(j)}^\top \right), \\ &= -\mathbf{\Omega}_\perp (2\mathbf{r} + \mathbf{e}_{k(j)}) \mathbf{e}_{k(j)}^\top. \end{aligned} \tag{S.29}$$

where the last step follows from the relation  $\mathbf{F}\mathbf{F}^+ \mathbf{F} = \mathbf{F}$ . In order to confirm convergence, we need to prove that the mean update  $\langle \Delta \mathbf{\Omega}_\perp \rangle_{\text{spikes}}$  always decreases the norm of  $\|\mathbf{\Omega}_\perp\|^2$ , i.e. we need to show that

$$\begin{aligned} \|\mathbf{\Omega}_\perp\|^2 &\geq \left\| \mathbf{\Omega}_\perp + \epsilon \langle \Delta \mathbf{\Omega}_\perp \rangle_{\text{spikes}} \right\|^2, \\ &= \|\mathbf{\Omega}_\perp\|^2 + 2\epsilon \text{tr} \left[ \mathbf{\Omega}_\perp^\top \langle \Delta \mathbf{\Omega}_\perp \rangle_{\text{spikes}} \right] + \mathcal{O}(\epsilon^2), \end{aligned}$$

which results in the inequality

$$0 \geq \text{tr} \left[ \mathbf{\Omega}_\perp^\top \langle \Delta \mathbf{\Omega}_\perp \rangle_{\text{spikes}} \right]. \tag{S.30}$$

---

<sup>15</sup>Note that (S.28) is a self-consistency relation since  $\mathbf{D}$  is also part of  $\hat{x}_i$ .

Plugging in (S.29) we find

$$\begin{aligned}
\text{tr} \left[ \mathbf{\Omega}_\perp^\top \langle \Delta \mathbf{\Omega}_\perp \rangle_{\text{spikes}} \right] &= -\text{tr} \left[ \mathbf{\Omega}_\perp^\top \left\langle \mathbf{\Omega}_\perp (2\mathbf{r} + \mathbf{e}_{k(j)}) \mathbf{e}_{k(j)}^\top \right\rangle_{\text{spikes}} \right], \\
&= -\text{tr} \left[ \mathbf{\Omega}_\perp \left\langle (2\mathbf{r} + \mathbf{e}_{k(j)}) \mathbf{e}_{k(j)}^\top \right\rangle_{\text{spikes}} \mathbf{\Omega}_\perp^\top \right], \\
&\approx -\text{tr} \left[ \mathbf{\Omega}_\perp \left\langle 2\mathbf{r}\mathbf{r}^\top / |\mathbf{r}| + \mathbf{e}_{k(j)} \mathbf{e}_{k(j)}^\top \right\rangle_{\text{spikes}} \mathbf{\Omega}_\perp^\top \right], \quad (\text{S.31})
\end{aligned}$$

where we used that for a given stimulus the rates are (to first order) fairly constant<sup>16</sup> over time and the average of the spike counts will be equivalent to the rates, so  $\langle \mathbf{r}\mathbf{e}_{k(j)}^\top \rangle_{\text{spikes}} \approx \langle \mathbf{r}\mathbf{r}^\top / |\mathbf{r}| \rangle_{\text{spikes}}$ . Finally, observe that the inner bracket of (S.31) is semi-positive definite and so we proved the desired relation  $\text{tr} \left[ \mathbf{\Omega}_\perp^\top \langle \Delta \mathbf{\Omega}_\perp \rangle_{\text{spikes}} \right] \leq 0$ . Consequently, any stable network will converge to a low-rank factorization under mild assumptions.

#### 4.4 Recurrent weights: Learning with L2 costs

As explained in section 3.5, we need to introduce quadratic costs before considering the learning of the feedforward weights. The quadratic (L2) costs change the target connectivity to  $\mathbf{\Omega} \rightarrow -\mathbf{F}\mathbf{D} - \mu\mathbf{I}$ . This target can be obtained through the following learning rule, modified from (S.24),

$$\Delta \mathbf{\Omega} \propto -2(\mathbf{V} + \mu\mathbf{r})\mathbf{e}_{k(j)}^\top - (\mathbf{\Omega} + \mu\mathbf{I})\mathbf{e}_{k(j)}\mathbf{e}_{k(j)}^\top,$$

or, without the burden of seeing through the matrix-vector notation,

$$\Delta \Omega_{nk} \propto \begin{cases} -2(V_n + \mu r_n) - \Omega_{nk} - \mu \delta_{nk} & \text{if } k \text{ spiked,} \\ 0 & \text{otherwise.} \end{cases}$$

We remind the reader that quantities such as the voltage or the instantaneous rate are here assumed to be evaluated directly *before* a spike of neuron  $k$ , i.e.,  $V_n = V_n^{\text{before}}(t_k)$  and  $r_n = r_n^{\text{before}}(t_k)$ . To show the fixed points of this modified learning rule, we follow the exact same analysis as in section 4.2, see (S.26),

$$\begin{aligned}
\Delta \mathbf{\Omega} &\propto -2(\mathbf{V} + \mu\mathbf{r})\mathbf{e}_{k(j)}^\top - (\mathbf{\Omega} + \mu\mathbf{I})\mathbf{e}_{k(j)}\mathbf{e}_{k(j)}^\top \\
&\stackrel{(\text{S.6})}{=} -2(\mathbf{F}\mathbf{x} + (\mathbf{\Omega} + \mu\mathbf{I})\mathbf{r})\mathbf{e}_{k(j)}^\top - (\mathbf{\Omega} + \mu\mathbf{I})\mathbf{e}_{k(j)}\mathbf{e}_{k(j)}^\top \\
&= -2\mathbf{F}\mathbf{x}\mathbf{e}_{k(j)}^\top - (\mathbf{\Omega} + \mu\mathbf{I})(2\mathbf{r} + \mathbf{e}_{k(j)})\mathbf{e}_{k(j)}^\top.
\end{aligned}$$

Compared to (S.26) we only replaced  $\mathbf{\Omega}$  by  $\mathbf{\Omega} + \mu\mathbf{I}$ . Consequently, all arguments concerning the fixed points  $-\mathbf{F}\mathbf{D}$  and convergence in section 4.2 and 4.3 now hold for  $\mathbf{\Omega} + \mu\mathbf{I}$ , and so we proved  $\mathbf{\Omega} \rightarrow -\mathbf{F}\mathbf{D} - \mu\mathbf{I}$ . Following the same argument, the fixed points (S.28) of the decoder do not change.

<sup>16</sup>Strictly speaking, this assumption is only valid in the limit of high instantaneous firing rates. In the regime of low firing rates, however, the (positive) diagonals in the inner bracket of (S.31) dominate and so the expectation value is still likely to be semi-positive definite as required to prove relation (S.30)

## 4.5 Feedforward weights: Learning rule

<sup>17</sup> In order to solve the full quadratic optimization problem (S.8) we need to ensure that the feedforward weights  $\mathbf{F}$  align with the decoder  $\mathbf{D}^\top$ . To this end, we remind the reader that the decoder will converge to (S.28),

$$\mathbf{D}_n = 2 \langle \mathbf{x} - \hat{\mathbf{x}} \rangle_{\text{n spikes}}.$$

In principle we would like to use this quantity to guide learning of the feedforward weights  $\mathbf{F}$ , just as we did in section 3.6. From a biophysical point of view, however, we cannot assume that the feedforward weights have access to the error  $\mathbf{x} - \hat{\mathbf{x}}$  (only to projections of the error). Fortunately the difference between  $\mathbf{x} - \hat{\mathbf{x}}$  will be proportional to the input signal  $\mathbf{x}$ , on average, since we assumed that the quadratic costs are non-negligible (see previous section). These costs will prohibit  $\hat{\mathbf{x}}$  to fully match the size of  $\mathbf{x}$ , an effect that increases linearly with the size of  $\mathbf{x}$ . Accordingly, input signal and error are, on average, proportional to each other, i.e.,  $\mathbf{x} - \hat{\mathbf{x}} \propto \mathbf{x}$ . The learning rule for the feedforward connections can therefore be approximated by:

$$\Delta \mathbf{F}_n(t_j) \propto \begin{cases} \mathbf{x}(t_j) - \mathbf{F}_n & \text{if } n \text{ spiked,} \\ 0 & \text{otherwise.} \end{cases} \quad (\text{S.32})$$

Importantly, we note that, if the current  $\mathbf{c}$  is changing slowly compared to the dynamics of the network, any sufficiently leaky integration of  $\mathbf{c}$  is a good approximation of  $\mathbf{x} - \hat{\mathbf{x}}$ . This observation becomes particularly important in the case of faster inputs: here the error  $\mathbf{x} - \hat{\mathbf{x}}$  can become dominated by the inability of the network to follow the inputs, so that a stable equilibrium is never reached. In such cases we often find numerically that a less leaky integration of the current leads to more efficient networks and better reconstruction errors. For the sake of mathematical precision, we will here make the assumption that  $\mathbf{c}$  is changing slowly, as also stated at the very beginning, section 1.1, and we will proceed with (S.32).

## 4.6 Feedforward weights: Fixed-point analysis

Analysing the stable fixed points from the interacting feedforward and recurrent synaptic plasticity rules is daunting since the membrane voltage of each cell depends on the exact sequence and timing of the spikes. Under these conditions there is little we can do beyond the numerical simulations (see main text). For large networks, however, even small noise sources will considerably randomise the timings and sequences of spikes [1], and so in this limit it makes sense to analyse the fixed points under the assumption that spikes are distributed according to an inhomogeneous Poisson process with mean firing rates  $\bar{r}_k(\mathbf{x})$ . In this case the fixed point of the feedforward learning rule, (S.32), is simply given by computing the expectation value over stimuli,

$$\mathbf{F}^* = \langle \bar{\mathbf{r}} \mathbf{x}^\top \rangle.$$

---

<sup>17</sup>THERE ARE PLENTY OF TRANSPOSES MISSING IN FF RULES HERE AND BELOW ... FIX !!!

Since the feedforward weights align with the decoder by design, the latter has the same fixed point (up to a transpose), so that

$$\mathbf{D}^* = \langle \mathbf{x} \bar{\mathbf{r}}^\top \rangle.$$

By multiplying with  $\mathbf{D}^{*\top} \mathbf{D}^*$  from the right we can identify a simple condition on the fixed point,

$$\begin{aligned} \mathbf{D}^* \mathbf{D}^{*\top} \mathbf{D}^* &= \langle \mathbf{x} \bar{\mathbf{r}}^\top \rangle \mathbf{D}^{*\top} \mathbf{D}^* \\ &= \langle \mathbf{x} (\mathbf{D}^* \bar{\mathbf{r}})^\top \rangle \mathbf{D}^* \\ &= \langle \mathbf{x} \hat{\mathbf{x}} \rangle \mathbf{D}^*. \end{aligned}$$

As observed above, the reconstruction  $\hat{\mathbf{x}}$  will closely follow the input signal  $\mathbf{x}$ , only slightly scaled down due to the quadratic costs. Since the input signal was assumed to be white,  $\langle \mathbf{x} \mathbf{x}^\top \rangle = \mathbf{I}$ , we can conclude that  $\langle \mathbf{x} \hat{\mathbf{x}} \rangle \propto \mathbf{I}$ . Hence,

$$\mathbf{D}^* \mathbf{D}^{*\top} \mathbf{D}^* \propto \mathbf{D}^*.$$

This condition is only fulfilled if the transpose of  $\mathbf{D}^*$  is its own pseudo-inverse, and so  $\mathbf{D}^*$  is a unitary matrix. (Or, more precisely, a slightly scaled down version of a unitary matrix.) In other words, in its fixed points the network represents the independent axes of a white stimulus on orthogonal directions of the population response  $\mathbf{r}$ , which is optimal. We discuss the non-whitened inputs in the section 4.8.

## 4.7 L1 cost and the scaling problem

<sup>18</sup> We have shown that under mild assumptions the combination of both learning rules will make the network converge to a  $\mathbf{F} \rightarrow \mathbf{D}^\top$  and  $\mathbf{\Omega} \rightarrow -\mathbf{D}^\top \mathbf{D} - \mu \mathbf{I}$ , similar to the optimal connectivity structure that we derived in section 1. So far, however, we have ignored the scaling of the synaptic connectivity, i.e. the relationship between the threshold  $T_n$  and the scale of the feedforward weights  $\mathbf{F}_n$  and the autapse  $\mathbf{\Omega}_{nn}$ , see section 2.4,

$$-\Omega_{nn} = \|\mathbf{D}_n\|_2^2 + \mu = 2T_n - \nu, \quad (\text{S.33})$$

$$\|\mathbf{F}_n\|_2^2 = 2T_n - \mu - \nu. \quad (\text{S.34})$$

Whereas the L2 cost modifies the recurrent connectivity, so that  $\mathbf{\Omega} \rightarrow -\mathbf{D}^\top \mathbf{D} - \mu \mathbf{I}$ , the L1 cost *only* enters the learning through these two equations. Since we assume that the thresholds of the neurons are given some initial value and are then never changed, our learning rules need to be modified in order to account for the appropriate scale of the synaptic weights. To guarantee the relation  $\Omega_{nn} = 2T_n - \nu$ , we introduce a scaling factor  $\beta_n$  for every neuron  $n$  in the learning rule of the recurrent synapses,

$$\Delta \Omega_{nk} \propto \begin{cases} -\beta_n(V_n + \mu r_n) - \Omega_{nk} - \mu \delta_{nk} & \text{if } k \text{ spiked,} \\ 0 & \text{otherwise.} \end{cases} \quad (\text{S.35})$$

---

<sup>18</sup>There are sign problems for the Omega in this section, when it comes to thresholds etc. Please fix.

Following again section 4.2 and the appropriate correction for the L2 costs in section 4.4, it is straight-forward to see that  $\mathbf{\Omega}$  will converge to  $-\mathbf{F}\mathbf{D}-\mu\mathbf{I}$ , where the decoder  $\mathbf{D}$  is now modified by the scaling factor  $\beta_n$  so that

$$D_{in} \rightarrow \beta_n \langle x_i - \hat{x}_i \rangle_{\text{n spikes}}.$$

Hence, in order to obey (S.33), the scaling factors  $\beta_n$  should evolve according to,

$$\begin{aligned} -\Omega_{nn} &= 2T_n - \nu \\ \Leftrightarrow \mathbf{F}_n \mathbf{D}_n + \mu &= 2T_n - \nu, \\ \Leftrightarrow \mathbf{F}_n \beta_n \langle \mathbf{x} - \hat{\mathbf{x}} \rangle_{\text{n spikes}} + \mu &= 2T_n - \nu, \\ \Leftrightarrow \beta_n &= \frac{2T_n - \mu - \nu}{\mathbf{F}_n^\top \langle \mathbf{x} - \hat{\mathbf{x}} \rangle_{\text{n spikes}}}, \\ \Leftrightarrow \beta_n &= \frac{2T_n - \mu - \nu}{T_n + \mu \langle r_n \rangle_{\text{n spikes}}} \end{aligned} \quad (\text{S.36})$$

<sup>19</sup> where in the last step we have used the relation  $\mathbf{F}_n^\top \langle \mathbf{x} - \hat{\mathbf{x}} \rangle_{\text{n spikes}} = \langle V_n \rangle_{\text{n spikes}} + \mu \langle r_n \rangle_{\text{n spikes}}$  and  $V_n = V_n^{\text{before}} = T_n$ , since the voltage directly before the spike of the firing neuron is, by definition, the neuron's threshold. Note that in the absence of costs,  $\mu = \nu = 0$ , we recover  $\beta_n = 2$ , i.e., the unscaled learning rule (S.22).

Similarly, to guarantee the scaling  $\|\mathbf{F}_n\|_2^2 = 2T_n - \mu - \nu$  of the feedforward weights, we introduce appropriate scaling factors  $\alpha_n$  into the learning rule (S.32),

$$\Delta \mathbf{F}_n \propto \begin{cases} \alpha_n \mathbf{x} - \mathbf{F}_n & \text{if } n \text{ spiked,} \\ 0 & \text{otherwise.} \end{cases} \quad (\text{S.37})$$

which will consequently lead to a scaling of the fixed point,

$$\mathbf{F}_n \rightarrow \alpha_n \langle \mathbf{x} \rangle_{\text{n spikes}}^\top.$$

Hence, in order to fulfill (S.34) it should hold that

$$\begin{aligned} \|\mathbf{F}_n\|^2 &= \mathbf{F}_n^\top \mathbf{F}_n \\ &= \mathbf{F}_n^\top \alpha_n \langle \mathbf{x} \rangle_{\text{n spikes}} \\ &= 2T_n - \mu - \nu \end{aligned}$$

from which we read off an expression for the scaling factors,

$$\alpha_n = \frac{2T_n - \mu - \nu}{\mathbf{F}_n^\top \langle \mathbf{x} \rangle_{\text{n spikes}}}. \quad (\text{S.38})$$

The learning rules (S.35) and (S.37) in conjunction with the definition of the scaling factors (S.36) and (S.38) are thus the set of rules that take into account all costs and will make the network converge to the optimal network configuration with the optimal decoding weights.

---

<sup>19</sup>Please check transposes on  $\mathbf{F}$  - some are wrong.

## 4.8 Non-whitened inputs

So far we have assumed that the input stimulus is zero-mean and whitened. To cover more general scenarios, we first revisit the optimal spiking neural network from section 1.7, following the approach outlined in [6] for rate networks. First, we note that a self-organized network is incapable of determining the true covariance of the signal (which could always be “arbitrarily” distorted by the feedforward weights) while the mean of the signal should be filtered out to increase efficiency (otherwise spikes are constantly emitted just to support a fixed offset). To take both aspects into account, we modify the loss function (S.10),

$$\ell = (\mathbf{x}_c - \mathbf{D}\mathbf{r})^\top \mathbf{C}^{-1} (\mathbf{x}_c - \mathbf{D}\mathbf{r}) + \mu \|\mathbf{r}\|^2 + \nu \|\mathbf{r}\|_1$$

where  $\mathbf{x}_c = \mathbf{x} - \bar{\mathbf{x}}$  is the mean signal and  $\mathbf{C} = \langle \mathbf{x}_c \mathbf{x}_c^\top \rangle$  is the signal covariance. In complete analogy to section 1.7, one can derive the voltages and thresholds of simple integrate-and-fire neurons,

$$\begin{aligned} \mathbf{V} &= \mathbf{D}^\top \mathbf{C}^{-1} \mathbf{x}_c - \mathbf{D}^\top \mathbf{C}^{-1} \mathbf{D} \mathbf{r} - \mu \mathbf{r}, \\ T_n &= \frac{1}{2} \left( \|\mathbf{D}_n\|^2 + \mu + \nu \right). \end{aligned}$$

Accordingly, the network is now characterized by feedforward weights  $\mathbf{F} = \mathbf{D}^\top \mathbf{C}^{-1}$  and recurrent weights  $\mathbf{\Omega} = -\mathbf{D}^\top \mathbf{C}^{-1} \mathbf{D} - \mu \mathbf{I} = -\mathbf{F} \mathbf{D} - \mu \mathbf{I}$ . These equations show that we only need to revisit the feedforward weights, whose relation to the decoder has changed, but not the recurrent weights, whose relation to the feedforward and decoder weights remains the same. Indeed, we did not make any (implicit or explicit) assumptions on the statistics of the input in the derivation of the recurrent learning rules, and so the same learning rule (S.35) applies in this case.

To make the feedforward weights converge to  $\mathbf{F} = \mathbf{D}^\top \mathbf{C}^{-1}$ , we ignore the correct scaling for now (see next section) and modify the learning rule (S.32) as

$$\Delta \mathbf{F}_n \propto \begin{cases} \mathbf{x}_c - \mathbf{F}_n^\top \mathbf{x}_c \mathbf{x}_c & \text{when neuron } n \text{ spikes,} \\ 0 & \text{otherwise.} \end{cases} \quad (\text{S.39})$$

We emphasize that this learning rule is still local. We can highlight this feature by stating the learning rule for the  $i$ -th element of  $\mathbf{F}_n$ ,

$$\Delta F_{in} \propto \begin{cases} [x_c]_i - (\mathbf{F}_n^\top \mathbf{x}_c)[x_c]_i & \text{when neuron } n \text{ spikes,} \\ 0 & \text{otherwise.} \end{cases}$$

Here,  $\mathbf{F}_n^\top \mathbf{x}_c$  is simply the total feedforward current that the postsynaptic neuron received. Accordingly, the modified learning rule requires a multiplicative, yet local interaction between the presynaptic signal,  $[x_c]_i$ , and the postsynaptic current. In Figure 4 of the main text, we simulate this modified learning rule in a network of 12 neurons that receive a correlated input signal. Interestingly, the network learns tuning curves that are narrower and denser around the most frequently presented signal directions. This is reminiscent of the tuning curves derived from efficient coding principles in population of poisson-firing neurons [20].

Following the derivation of section 4.6, and assuming once more Poisson-distributed spike trains, the fixed points,  $\mathbf{F}^*$ , of the feedforward rule become

$$\begin{aligned}\langle \bar{\mathbf{r}} \mathbf{x}_c^\top - \mathbf{F}^* \mathbf{x}_c \mathbf{x}_c^\top \rangle &= 0, \\ \Leftrightarrow \mathbf{F}^* \langle \mathbf{x}_c \mathbf{x}_c^\top \rangle &= \langle \bar{\mathbf{r}} \mathbf{x}_c^\top \rangle, \\ \Rightarrow \mathbf{F}^* &= \mathbf{D}^{*\top} \mathbf{C}^{-1}.\end{aligned}$$

where the fixed point of the decoder,  $\mathbf{D}^*$  remains untouched, and becomes

$$\mathbf{D}^* \propto \langle \mathbf{x}_c \bar{\mathbf{r}}^\top \rangle.$$

Using this relation once more, and multiplying it with  $\mathbf{D}^{*\top} \mathbf{C}^{-1} \mathbf{D}^*$  from the right, we find the following relation for the decoder

$$\begin{aligned}\mathbf{D}^* \mathbf{D}^{*\top} \mathbf{C}^{-1} \mathbf{D}^* &\propto \langle \mathbf{x}_c \bar{\mathbf{r}}^\top \rangle \mathbf{D}^{*\top} \mathbf{C}^{-1} \mathbf{D}^*, \\ &= \langle \mathbf{x}_c (\mathbf{D}^* \bar{\mathbf{r}})^\top \rangle \mathbf{C}^{-1} \mathbf{D}^*, \\ &= \langle \mathbf{x}_c \hat{\mathbf{x}}_c \rangle \mathbf{C}^{-1} \mathbf{D}^*, \\ &\propto \mathbf{D}^*,\end{aligned}$$

which is fulfilled if  $\mathbf{D}^* = \mathbf{C}^{1/2} \mathbf{U}$ , where  $\mathbf{U}$  is a unitary matrix. Then  $\mathbf{F}^* = \mathbf{D}^{*\top} \mathbf{C}^{-1} = \mathbf{U}^\top \mathbf{C}^{-1/2}$ . This last equation exposes the solution that the network finds: it whitens the input through its feedforward filters before encoding it along orthogonal axis in the population response.

#### 4.9 Simplifying assumptions for the main paper

The scaling factors  $\alpha_n$  and  $\beta_n$  for the feedforward and recurrent weights guarantee the convergence of the network to the properly scaled weights. It is important to remember that the scaling factors only set the right scale of the weights, they do not affect the overall structure of the optimal connectivities,  $\mathbf{F} \propto \mathbf{D}^\top$  and  $\mathbf{\Omega} \propto -\mathbf{D}^\top \mathbf{D} - \mu \mathbf{I}$ . In practice, we set all thresholds to the same values  $T_n = T$ . In addition, we note that fixing the scaling factors  $\alpha_n$  and  $\beta_n$  merely fixes a set of fixed points with a particular L1 cost  $\nu$  and scaling of  $\mathbf{D}$ . To ease simulation we fix two scaling factors  $\alpha = \alpha_n$  and  $\beta = \beta_n$  by hand such that the fixed points exhibit reasonable cost values and scales. This approximation worked quite well. The recurrent learning rule, (S.35), then becomes

$$\Delta \Omega_{nk} \propto \begin{cases} -\beta(V_n + \mu r_n) - \Omega_{nk} - \mu \delta_{nk} & \text{if } k \text{ spiked,} \\ 0 & \text{otherwise.} \end{cases} \quad (\text{S.40})$$

which is the equation shown in the main paper. The feedforward rule, (S.37), becomes

$$\Delta F_{in} \propto \begin{cases} \alpha x_i - F_{in} & \text{if } n \text{ spiked,} \\ 0 & \text{otherwise.} \end{cases} \quad (\text{S.41})$$

In both rules,  $\alpha$  and  $\beta$  are simply treated as free parameters.

## 5 Learning in the E/I network

So far we neglected Dale’s law, i.e. the distinction between excitatory and inhibitory neurons. Using the intuition built up in the last three sections it is straight-forward to see how learning in an E/I network should proceed. Consider a population of excitatory neurons that receives feedforward input. E-E connections are constrained to be excitatory, and so neurons with overlapping inputs cannot balance each other. If, however, a population of inhibitory neurons has learned to represent the signal encoded by the excitatory population, then its representation can in turn be used to balance the excitatory population. This suggests that the E-I connections are to be treated like feedforward connections because the excitatory population response serves as the input to the inhibitory population. The E-E and I-I connections are to be trained by the recurrent learning rule since they aim to balance the E- and the I-population respectively. Finally, the I-E connections should be trained the same way since they aim to balance the E-population.

We can formalize this intuition as follows. First, consider the optimal network without costs,  $\mathbf{\Omega} = -\mathbf{D}\mathbf{D}^\top$ , and split the decoder weights  $\mathbf{D} = \mathbf{D}_+ - \mathbf{D}_-$  into one part with all positive and another with the absolute value of all negative entries. Then,

$$\begin{aligned}\mathbf{\Omega}\mathbf{r} &= -(\mathbf{D}_+ - \mathbf{D}_-)^\top(\mathbf{D}_+ - \mathbf{D}_-)\mathbf{r}, \\ &= (\mathbf{D}_-^\top\mathbf{D}_+ + \mathbf{D}_+^\top\mathbf{D}_-)\mathbf{r} - (\mathbf{D}_+^\top\mathbf{D}_+ + \mathbf{D}_-^\top\mathbf{D}_-)\mathbf{r}.\end{aligned}$$

We can identify the first term as the recurrent excitation and the second term as the recurrent inhibition. It is this latter term that we need to approximate by means of an inhibitory population. To this end let  $\mathbf{r}$  be approximated by the response  $\mathbf{s}$  of a second population, i.e.  $\hat{\mathbf{r}} = \tilde{\mathbf{D}}\mathbf{s}$  and so

$$\mathbf{\Omega}\mathbf{r} \approx (\mathbf{D}_-^\top\mathbf{D}_+ + \mathbf{D}_+^\top\mathbf{D}_-)\mathbf{r} - (\mathbf{D}_+^\top\mathbf{D}_+ + \mathbf{D}_-^\top\mathbf{D}_-)\tilde{\mathbf{D}}\mathbf{s}.$$

The second population shall minimize the objective

$$L_I = \arg \min_{\tilde{\mathbf{D}}} \left\langle \left\| \mathbf{r} - \tilde{\mathbf{D}}\mathbf{s} \right\|^2 \right\rangle,$$

which we know is solved optimally by a network with feedforward weights  $\tilde{\mathbf{D}}^\top$  and recurrent weights  $-\tilde{\mathbf{D}}\tilde{\mathbf{D}}^\top$ . Observe that this second population has only inhibitory recurrent weights and its influence on the first is solely inhibitory; it can therefore be identified as an inhibitory population. At the same time, the first population has only excitatory recurrent weights and its influence on the second is solely excitatory; it can therefore be identified as an excitatory population.

In summary, the structure of the optimal E/I network is given by feedforward weights  $\mathbf{D}^\top$ , E-E connections  $\mathbf{\Omega}_{EE} = \mathbf{D}_-^\top\mathbf{D}_+ + \mathbf{D}_+^\top\mathbf{D}_-$ , E-I connections  $\mathbf{\Omega}_{IE} = \tilde{\mathbf{D}}^\top$ , I-I connections  $\mathbf{\Omega}_{II} = -\tilde{\mathbf{D}}\tilde{\mathbf{D}}^\top$  and I-E connections  $\mathbf{\Omega}_{EI} = -(\mathbf{D}_+^\top\mathbf{D}_+ + \mathbf{D}_-^\top\mathbf{D}_-)\tilde{\mathbf{D}}$ . From the derivation it is clear that  $\mathbf{\Omega}_{IE}$  act as feedforward weights to the inhibitory population and are thus to be trained by the standard feedforward rule. All other weights, i.e.  $\mathbf{\Omega}_{EE}$ ,  $\mathbf{\Omega}_{IE}$  and  $\mathbf{\Omega}_{EI}$ , are trained using the recurrent learning rule. The training then proceeds as in the non-Dale’s case except for the sign constraint on the synaptic weights.

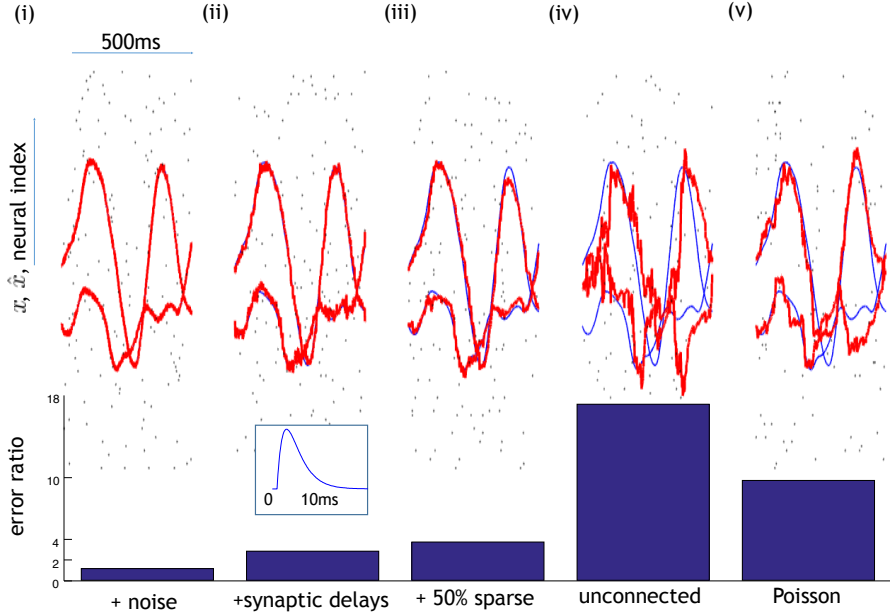

**Figure S1:** Robustness of the framework to noise, synaptic delays, and missing connections. Spike trains (black dots) of 60 neurons (out of a total of 200), input signals (thin blue lines), network estimates (thick red lines), and error ratio between the perturbed and optimal networks after learning. (i) White noise current is injected into each neuron. (ii) In addition to the injected noise, synaptic input currents are modeled with a realistic post-synaptic potential, including a transmission delay (inset). (iii) In addition to noise and realistic synapses, 50% of the recurrent connections are randomly removed. (iv) All recurrent connections are removed so that the network is now composed of unconnected leaky integrate and fire neurons. (v) A population of independent Poisson-firing neurons with instantaneous firing rates identical to the network in (i), but without learning.

## 6 Robustness of learning

When deriving the learning rules, we have assumed a network of largely idealistic, noise-free integrate-and-fire neurons that are fully connected. One may therefore wonder to what extent the learning rules generalize systems that deviate from this idealized scenario. To demonstrate the robustness of the learning rules, we therefore trained networks with various sub-optimal properties, such as increased levels of noise, realistic synaptic delays, or sparser connectivities. We then compared the performance of these suboptimal networks with the corresponding optimal networks.

We trained networks of  $N = 200$  neurons to optimally encode two uncorrelated, time-varying inputs. The initialization of the feedforward and recurrent weights were identical in all cases. We adjusted the neural firing thresholds to achieve identical (final) population firing rates for all the networks. To compare the performance of the suboptimal networks to the optimal network, we computed the error ratio, defined as the ratio of the network mean reconstruction

error, and the reconstruction error of the optimal network. Thus, a relative error of 1.5 implies that the performance is 50% worse than optimal.

We first simulated a network with relatively large membrane voltage noise (Figure S1(i)). The learning rules worked just as well as before. However, the addition of the noise caused a small increase in the error of the learnt network compared to a noise-free network.

In Figure S1(ii), we added a more realistic synapse model to the network from Figure S1(i). More specifically, we replaced each spike by a synaptic filter  $h(t) = (t/\tau^2 \exp -(t/\tau)$  with  $\tau = 3\text{ms}$ , and we added a fixed transmission delay of  $\delta t = 0.5\text{ms}$  to each spike. The learning again worked well, but the overall final error of the network was larger than before.

In Figure S1(iii), we also removed 50% of the recurrent connections at random, i.e., we set these connections to zero and did not learn them. This caused a four-fold increase in the final error of the network compared to the optimal network. Despite this overall increase in the error, however, these degraded networks still outperform a network of independent integrate-and-fire neurons (Figure S1(iv)) or independent Poisson firing neurons (Figure S3(v)). Accordingly, the learning of the feedforward and recurrent connectivity still improves the performance of the network, even under these highly constrained scenarios.

## 7 Learning a Speech signal, Supplementary results

This section provides additional results for the network trained with speech signals (Figure 5 and 6 in main paper). Here, we report the initial, learnt, and re-trained input and decoding weights. We also show the result of re-learning a new sound when training the feed-forward, but not the recurrent connections.

## 8 Numerical Simulations

### 8.1 Network Dynamics

The membrane voltage  $V_n$  of each cell is simulated according to a discrete-time (Euler) approximation of the differential equations, (S.5), (S.3), and (S.4),

$$V_n(t + \Delta t) = V_n(t) + \Delta t \Delta V_n(t)$$

In Figure 2 and 3, the target signal  $\mathbf{x}(t)$  is set as follows: we first draw a random vector  $\mathbf{y}(t) \in \mathbf{R}^I$  from a zero-mean Gaussian distribution  $\mathbf{y}(t) \sim \mathcal{N}(0, \sigma^2 \mathbf{I})$  for every time-step  $t$  and then convolve  $\mathbf{y}(t)$  with a Gaussian kernel of size  $\eta$  over time to get  $\mathbf{x}(t)$ . For Figure 5, the target signal was the speech spectrogram, sampled at 100Hz and interpolated to reach a temporal resolution of 0.05 ms. The input current  $\mathbf{c}(t)$  is computed following (S.1), i.e.,

$$c_i(t) = \dot{x}_i(t) + \lambda x_i(t).$$

To randomize the spikes, gaussian noise terms  $\xi_V$  and  $\xi_T$  with very small variances and zero means are added respectively to the voltage equation and to the threshold of the neurons.

In all simulations, the recurrent (and I to E) weights are trained by means of the recurrent learning rule (S.40).

The feedforward weights  $\mathbf{F}$  and the  $E-I$  connection follows (S.41) (whitened inputs, Figure 2 and 3) or (S.39) (non-whitened input, Figure 4–6). However, in Figure 3–6, the input signal  $\mathbf{x}$  in equations (S.41) and (S.39) is replaced by the input currents integrated with a larger leak term  $\lambda_F > \lambda$ . For example, in Figure 3, the learning rule of the feedforward connection is

$$\Delta \mathbf{F}_n(t_j) \propto \begin{cases} \bar{\mathbf{c}}(t_j) - \mathbf{F}_n & \text{if } n \text{ spiked,} \\ 0 & \text{otherwise.} \end{cases}$$

where  $\bar{\mathbf{c}}$  obeys  $\dot{\bar{\mathbf{c}}} = -\lambda_F \bar{\mathbf{c}} + \mathbf{c}$ .

The constant scaling term  $\alpha$  is chosen so as to achieve mean firing rates of around 5 to 10 Hz after training. The learning rates  $\epsilon_F$  and  $\epsilon_\Omega$  of the feedforward and recurrent weights are either kept constant throughout the simulation (Figures 2–4), or progressively decreased (Figure 5). Importantly, there is a separation of time-scales such that  $\epsilon_\Omega = 10\epsilon_F$ ; this ensures that the network is always kept in a balanced (and thus stable) regime throughout learning.

The full pseudo-code for the non-Dales case can be found in algorithm 1.

## 8.2 Initialization

To initialize the feedforward weights  $\mathbf{F} \in \mathbb{R}^{N \times I}$ , we first draw all elements from a zero-mean normal distribution,  $\mathbf{F}_{ni} \sim \mathcal{N}(0, 1)$ , and then normalize each row to be of length  $\gamma$ , i.e.

$$F_{ni} \rightarrow \gamma \frac{F_{ni}}{\sqrt{\sum_i F_{ni}^2}}.$$

In Figures 2, and 4–6 the initial recurrent weights  $\mathbf{\Omega} \in \mathbb{R}^{N \times N}$  are proportional to the unit matrix  $\mathbf{I}_N$  with proportionality  $\omega$ , i.e.  $\mathbf{\Omega}_0 = \omega \mathbf{I}_N$ . This simplified initialization is chosen for illustrative purposes; the learning also works for more general, random initializations of the recurrent connections. The recurrent connectivity in the E/I network (Figure 3) is similarly initialized as  $\mathbf{\Omega}_{EE} = \omega_{EE} \mathbf{I}_{N_E}$  and  $\mathbf{\Omega}_{II} = \omega_{II} \mathbf{I}_{N_I}$ . In all simulations there are four times more excitatory than inhibitory neurons,  $N_E = 4 \cdot N_I$ , and so we initialize the E-I and I-E connections according to  $\mathbf{\Omega}_{EI} = \omega_{EI} [\mathbf{I}_{N_I}, \mathbf{I}_{N_I}, \mathbf{I}_{N_I}, \mathbf{I}_{N_I}]$  and  $\mathbf{\Omega}_{IE} = \omega_{IE} [\mathbf{I}_{N_I}, \mathbf{I}_{N_I}, \mathbf{I}_{N_I}, \mathbf{I}_{N_I}]^\top$  where the squared brackets denote a stacking of the elements along the rows. The thresholds  $T_n = T$  are kept constant (except for Figure 5,6) over the course of the simulation (including learning) and are homogeneous across cells.

## 8.3 Tuning Curves

To compute the tuning curves (Figures 2–4), we define a circle in a 2D plane and then sample inputs uniformly on this circle. For each trial a constant input (orientation) is sampled from this circle and presented to the network (running without plasticity). At the end of the trial, the average firing rate of each neuron is computed over all the duration of the presentation of the input except for the initial transient period.

---

**Algorithm 1** Pseudo-code for simulation of non-Dale's network (Figures 2, 4–6)

---

```

1: procedure SIMULATION
2:    $N, I \leftarrow$  number of cells and input dimensions
3:    $\lambda \leftarrow$  membrane leak
4:    $\mathbf{F}(0) \leftarrow$  initial feedforward weights
5:    $\mathbf{\Omega}(0) \leftarrow$  initial recurrent weights
6:    $S \leftarrow$  total simulation time
7:    $dt \leftarrow$  time-step
8:    $\epsilon_F, \epsilon_\Omega \leftarrow$  learning rates
9:    $\alpha, \beta \leftarrow$  scaling factors in learning equations
10:   $\mu \leftarrow$  L2 cost
11:   $T \leftarrow$  threshold
12:   $\sigma, \eta \leftarrow$  standard deviation of signal, time-scale of smoothing kernel
13:  top:
14:     $\mathbf{V}(0) \leftarrow \mathbf{0}$  (initial voltage)
15:     $\mathbf{o}(0) \leftarrow \mathbf{0}$  (initial spikes)
16:     $\mathbf{r}(0) \leftarrow \mathbf{0}$  (initial filtered spikes)
17:     $\Gamma \leftarrow$  closest integer to  $S/dt$  (number of simulation steps)
18:     $\mathbf{x}(\tau) \leftarrow$  drawn from  $\mathcal{N}(0, \sigma^2 \mathbf{I}_I)$  for all  $\tau = 1 \dots \Gamma$ 
19:     $\mathbf{x}(\tau) \leftarrow \mathbf{x}(\tau)$  filtered with Gaussian kernel of width  $\eta$  over time
20:     $\xi_V(\tau) \leftarrow$  drawn from  $\mathcal{N}(0, \sigma_{\xi_V}^2 \mathbf{I}_N)$  for all  $\tau = 1 \dots \Gamma$ 
21:     $\xi_T(\tau) \leftarrow$  drawn from  $\mathcal{N}(0, \sigma_{\xi_T}^2 \mathbf{I}_N)$  for all  $\tau = 1 \dots \Gamma$ 
22:  loop:
23:    for  $\tau = 1$  to  $\Gamma$  do
24:       $\mathbf{c}(\tau - 1) = \mathbf{x}(\tau) - \mathbf{x}(\tau - 1) + \lambda dt \mathbf{x}(\tau - 1)$ 
25:       $\mathbf{V}(\tau) = (1 - \lambda dt) \mathbf{V}(\tau - 1) + dt \mathbf{F}(\tau - 1)^\top \mathbf{c}(\tau - 1) + \mathbf{\Omega}(\tau - 1) \mathbf{o}(\tau - 1) + \xi_V(\tau)$ 
26:
27:       $\mathbf{o}(\tau) = \mathbf{0}$ 
28:       $n \leftarrow \arg \max (\mathbf{V} - \mathbf{T}) - \xi_T(\tau)$ 
29:      if  $V_n > T_n$  then
30:         $o_n(\tau) = 1$ 
31:         $\mathbf{F}_n(\tau) = \mathbf{F}_n(\tau - 1) + \epsilon_F (\alpha \mathbf{x}(\tau - 1) - \mathbf{F}_n(\tau - 1))$ 
32:         $\mathbf{\Omega}_n(\tau) = \mathbf{\Omega}_n(\tau - 1) - \epsilon_\Omega (\beta (\mathbf{V}(\tau - 1) + \mu \mathbf{r}(\tau - 1)) + \mathbf{\Omega}_n(\tau - 1))$ 
33:         $\Omega_{nn}(\tau) = \Omega_{nn}(\tau - 1) - \epsilon_\Omega \mu$ 
34:
35:       $\mathbf{r}(\tau) = (1 - \lambda dt) \mathbf{r}(\tau - 1) + \mathbf{o}(\tau - 1)$ 

```

---

---

**Algorithm 2** Pseudo-code for simulation of Dales network (Figure 3)

---

```

1: procedure SIMULATION
2:    $N_E, N_I, I \leftarrow$  number of cells in the excitatory and inhibitory populations and input dimensions
3:    $\lambda, \lambda_F, \lambda_{EI} \leftarrow$  membrane leak and integration time constants for the FF learning rule
4:    $\mathbf{F}(0) \leftarrow$  initial feedforward weights
5:    $\mathbf{\Omega}^{EE}(0), \mathbf{\Omega}^{EI}(0), \mathbf{\Omega}^{II}(0), \mathbf{\Omega}^{IE}(0) \leftarrow$  initial recurrent weights
6:    $S \leftarrow$  total simulation time
7:    $dt \leftarrow$  time-step
8:    $\epsilon_F, \epsilon_\Omega \leftarrow$  learning rates
9:    $\alpha, \beta \leftarrow$  scaling factors in learning equations
10:   $\mu \leftarrow$  L2 cost
11:   $T^E, T^I \leftarrow$  threshold
12:   $\sigma, \eta \leftarrow$  standard deviation of signal, time-scale of smoothing kernel
13:   $R^E, R^I \leftarrow$  refractory periods of the excitatory and inhibitory neurons
14:  top:
15:     $\mathbf{V}^E(0), \mathbf{V}^I(0) \leftarrow \mathbf{0}$  (initial voltage)
16:     $\mathbf{o}^E(0), \mathbf{o}^I(0) \leftarrow \mathbf{0}$  (initial spikes)
17:     $\mathbf{r}^E(0), \mathbf{r}^I(0) \leftarrow \mathbf{0}$  (initial filtered spikes)
18:     $\mathbf{R}^E(0), \mathbf{R}^I(0) \leftarrow \mathbf{0}$  (initial refractory periods spikes)
19:     $\Gamma \leftarrow$  closest integer to  $S/dt$  (number of simulation steps)
20:     $\mathbf{x}(\tau) \leftarrow$  drawn from  $\mathcal{N}(0, \sigma^2 \mathbf{I}_I)$  for all  $\tau = 1 \dots \Gamma$ 
21:     $\mathbf{x}(\tau) \leftarrow \mathbf{x}(\tau)$  filtered with Gaussian kernel of width  $\eta$  over time
22:     $\xi_E^V(\tau), \xi_I^V(\tau) \leftarrow$  drawn from  $\mathcal{N}(0, \sigma_{\xi_V}^2 \mathbf{I}_N)$  for all  $\tau = 1 \dots \Gamma$ 
23:     $\xi_E^T(\tau), \xi_I^T(\tau) \leftarrow$  drawn from  $\mathcal{N}(0, \sigma_{\xi_T}^2 \mathbf{I}_N)$  for all  $\tau = 1 \dots \Gamma$ 
24:    loop:
25:      for  $\tau = 1$  to  $\Gamma$  do
26:         $\mathbf{c}(\tau - 1) = \mathbf{x}(\tau) - \mathbf{x}(\tau - 1) + \lambda dt \mathbf{x}(\tau - 1)$ 
27:         $\mathbf{c}_E(\tau) = (1 - \lambda_F dt) \mathbf{c}_E(\tau - 1) + \mathbf{c}(\tau - 1)$ 
28:         $\mathbf{c}_I(\tau) = (1 - \lambda_{EI} dt) \mathbf{c}_E(\tau - 1) + \mathbf{o}_E(\tau - 1)$ 
29:         $\mathbf{V}^E(\tau) = (1 - \lambda dt) \mathbf{V}^E(\tau - 1) + dt \mathbf{F}(\tau - 1)^\top \mathbf{c}(\tau - 1) + \mathbf{\Omega}^{EE}(\tau - 1) \mathbf{o}^E(\tau - 1) + \mathbf{\Omega}^{IE}(\tau - 1) \mathbf{o}^I(\tau - 1) + \xi_E^V(\tau)$ 
30:
31:         $\mathbf{o}^E(\tau) = \mathbf{0}$ 
32:         $n_E \leftarrow \arg \max \left( \mathbf{V}^E - \mathbf{T}^E \right) - \xi_E^T(\tau)$ 
33:        if  $V_{n_E}^E > T_{n_E}^E \ \& \ R_{n_E}^E(\tau - 1) < 0$  then
34:           $\mathbf{o}_{n_E}^E(\tau) = 1$ 
35:           $R_{n_E}^E(\tau - 1) = R_{max}^E$ 
36:           $\mathbf{F}_{n_E}(\tau) = \mathbf{F}_{n_E}(\tau - 1) + \epsilon_F (\alpha \mathbf{c}_E(\tau - 1) - \mathbf{F}_{n_E}(\tau - 1))$ 
37:           $\mathbf{\Omega}_{n_E}^{EE}(\tau) = \mathbf{\Omega}_{n_E}^{EE}(\tau - 1) - \epsilon_\Omega (\beta (\mathbf{V}^E(\tau - 1) + \mu \mathbf{r}^E(\tau - 1)) + \mathbf{\Omega}_{n_E}^{EE}(\tau - 1))$ 
38:           $\mathbf{\Omega}_{n_E}^{EE}(\tau) = \mathbf{\Omega}_{n_E}^{EE}(\tau) - \epsilon_\Omega \mu$ 
39:           $\mathbf{\Omega}_{n_E}^{EI}(\tau) = \mathbf{\Omega}_{n_E}^{EI}(\tau - 1) - \epsilon_\Omega (\beta (\mathbf{V}^I(\tau - 1) + \mu \mathbf{r}^I(\tau - 1)) + \mathbf{\Omega}_{n_E}^{EI}(\tau - 1))$ 
40:
41:           $R^E(\tau) = R^E(\tau - 1) - 1$ 
42:           $\mathbf{r}^E(\tau) = (1 - \lambda dt) \mathbf{r}^E(\tau - 1) + \mathbf{o}^E(\tau - 1)$ 

```

---

---

```

43:       $\mathbf{V}^I(\tau) = (1 - \lambda dt)\mathbf{V}^I(\tau - 1) + \mathbf{\Omega}^{EI}(\tau)\mathbf{o}^E(\tau) + \mathbf{\Omega}^{II}(\tau - 1)\mathbf{o}^I(\tau - 1) +$ 
       $\xi_I^V(\tau)$ 
44:
45:       $\mathbf{o}^I(\tau) = \mathbf{0}$ 
46:       $n_I \leftarrow \arg \max \left( \mathbf{V}^I - \mathbf{T}^I \right) - \xi_I^T(\tau)$ 
47:      if  $V_{n_I}^I > T_{n_I}^I$  &  $R_{n_I}^I(\tau - 1) < 0$  then
48:           $o_{n_I}^I(\tau) = 1$ 
49:           $R_{n_I}^I(\tau - 1) = R_{max}^I$ 
50:           $\mathbf{\Omega}_{n_I}^{EI}(\tau) = \mathbf{\Omega}_{n_I}^{EI}(\tau - 1) + \epsilon_F(\alpha \mathbf{c}_I(\tau - 1) - \mathbf{\Omega}_{n_I}^{EI}(\tau - 1))$ 
51:           $\mathbf{\Omega}_{n_I}^{II}(\tau) = \mathbf{\Omega}_{n_I}^{II}(\tau - 1) - \epsilon_\Omega(\beta(\mathbf{V}^I(\tau - 1) + \mu \mathbf{r}^I(\tau - 1)) + \mathbf{\Omega}_{n_I}^{II}(\tau - 1))$ 
52:           $\Omega_{n_I n_I}^{II}(\tau) = \Omega_{n_I n_I}^{II}(\tau - 1) - \epsilon_\Omega \mu$ 
53:           $\mathbf{\Omega}_{n_I}^{IE}(\tau) = \mathbf{\Omega}_{n_I}^{IE}(\tau - 1) - \epsilon_\Omega(\beta(\mathbf{V}^E(\tau - 1) + \mu \mathbf{r}^E(\tau - 1)) + \mathbf{\Omega}_{n_I}^{IE}(\tau - 1))$ 
54:
55:       $R^I(\tau) = R^I(\tau - 1) - 1$ 
56:       $\mathbf{r}^I(\tau) = (1 - \lambda dt)\mathbf{r}^I(\tau - 1) + \mathbf{o}^I(\tau - 1)$ 

```

---

| Parameters                                                 | Figure 2              | Figure 3                                                                                     | Figure 5,6                   |
|------------------------------------------------------------|-----------------------|----------------------------------------------------------------------------------------------|------------------------------|
| Number of neurons $N$                                      | 20                    | $N_E = 300/60$ (BC/D)<br>$N_I = 75/15$ (BC/D)                                                | 64                           |
| Dimension of input $I$                                     | 2                     | 3                                                                                            | 25                           |
| Time step $dt$                                             | $10^{-3}\text{s}$     | $10^{-4}\text{s}$                                                                            | $6.25 \cdot 10^{-5}\text{s}$ |
| Membrane leak $\lambda$                                    | $50 \text{ s}^{-1}$   | $50 \text{ s}^{-1}$                                                                          | $8 \text{ s}^{-1}$           |
| Integration time constant for the FF learning rule         | $\lambda_F = \lambda$ | $\lambda_F = 6\lambda$<br>$\lambda_{E-I} = \lambda$                                          | $\lambda_F = 125\lambda$     |
| Standard deviation of input $\sigma$                       | $2 \cdot 10^3$        | $2 \cdot 10^3$                                                                               | -                            |
| Time scale of input kernel $\eta$                          | 6 ms                  | 6 ms                                                                                         | -                            |
| Threshold $T$                                              | 0.5                   | 0.5                                                                                          | dynamic                      |
| standard deviation of the voltage noise $\sigma_{\xi_V}$   | $10^{-3}$             | $10^{-3}$                                                                                    | 0                            |
| standard deviation of the threshold noise $\sigma_{\xi_T}$ | $2 \cdot 10^{-2}$     | $2 \cdot 10^{-2}$                                                                            | $5 \cdot 10^{-3}$            |
| Learning rate $\epsilon_\Omega$                            | $10^{-4}$             | $10^{-4}$                                                                                    | variable                     |
| Learning rate $\epsilon_F$                                 | $10^{-5}$             | $10^{-5}$                                                                                    | variable                     |
| Scaling factor $\alpha$                                    | 0.21                  | 0.21                                                                                         | 1                            |
| Scaling factor $\beta$                                     | 1.25                  | 1                                                                                            | 1                            |
| L2 cost $\mu$                                              | 0.02                  | $\mu_E = 0.02, \mu_I = 0$                                                                    | 0.1                          |
| Initial scale $\gamma$                                     | 0.8                   | 1                                                                                            | -                            |
| Initial scale $\omega$                                     | -0.5                  | $\omega_{EE} = -0.02$<br>$\omega_{II} = -0.5$<br>$\omega_{EI} = 0.5$<br>$\omega_{IE} = -0.3$ | -                            |

**Table 1:** Simulation parameters for all simulations.

## 8.4 Fano Factor and Coefficient of Variation

The Fano factor and the coefficient of variation are computed as follows. A random direction is chosen in the input space and presented multiple times to the network (running without plasticity). For each trial the spike count  $c$  of the neurons is computed. then we compute the the Fano factor for each neuron using the formula :

$$F_n = \frac{\sigma_{c(n)}^2}{\mu_{c(n)}}$$

$\sigma_{c(n)}^2$  and  $\mu_{c(n)}$  are respectively the standard deviation and the mean of the the spike count of neuron  $n$ . This procedure is repeated using different random input directions. The final Fano factor is an average over the input directions and the neurons in the population.

The Coefficient of variation (CV) is computed using the same inputs. For each trial, instead of the spike count, we pool the interspike intervals (ISI) of all neurons. The formula used to compute the CV is

$$CV = \frac{\sigma_{ISI}}{\mu_{ISI}}$$

As for the Fano factor, the final CV is an average over the different input directions.

## 8.5 Learning the Speech Signal

To learn the speech signal (Figure 5,6), slight modifications were added to the previous learning scheme. In a non-whitened scenario, partial learning of the inhibitory recurrent connections can result in a large proportion of completely silent neurons. Since plasticity require pre- and post-synaptic spiking, these neuron never "recover" or participate in the representation. To avoid this issue, we used a dynamic threshold that decreases for unresponsive neuron and increases for neurons that are too active. The threshold decreased by  $-\epsilon_F$  for a neuron that did not fire any spike in a sliding window of 2.5s, and increased by  $\epsilon_F$  if its firing rate exceeded 20Hz in the last 2.5s. After about 1000 iterations, the firing rates are always maintained between these two bounds and the thresholds remain constant for the rest of the learning.

In Figures 5,6 the initial recurrent and feedforward weights are drawn from a normal distribution with standard deviations of 0.1 and 0.02 for the feedforward and the recurrent weights respectively; These initial weights are not normalized. The diagonal elements of the recurrent connectivity matrix (the resets) are equal to -0.8. Such strong inhibitory autapses insure the stability of the network in the initial state. In order to speed-up learning we used initially large learning rates ( $\epsilon_\Omega = 10^{-2}$ ,  $\epsilon_F = 10^{-3}$ ) that were progressively decreased to  $\epsilon_\Omega = 10^{-4}$  and  $\epsilon_F = 10^{-5}$ . For re-training to the new non-speech stimulus, we used the learning rates  $\epsilon_\Omega = 10^{-2}$ ,  $\epsilon_F = 10^{-3}$ . For re-training the feed-forward connections without the lateral connections, we used  $\epsilon_F = \frac{1}{4}10^{-2}$ ).

## References

- [1] Martin Boerlin, Christian K. Machens, Sophie Denève. *Predictive Coding of Dynamical Variables in Balanced Spiking Networks*. PLoS Comput Biol 9(11) (2013): e1003258.
- [2] Ralph Bourdoukan, David G.T. Barrett, Christian K. Machens, and Sophie Denève. *Learning Optimal Spike-based Representations*. Advances in Neural Information Processing Systems 25 (2012).
- [3] Peter Dayan and Larry F. Abbott. *Theoretical Neuroscience: Computational and Mathematical Modeling of Neural Systems*. MIT Press (2005).
- [4] Christopher J. Rozell, Don H. Johnson, Richard G. Baraniuk, and Bruno A. Olshausen. *Sparse coding via thresholding and local competition in neural circuits*. Neural Computation 20.10 (2008): 2526–2563
- [5] Joel Zylberberg, Jason T. Murphy, and Michael R. DeWeese. *A sparse coding model with synaptically local plasticity and spiking neurons can account for the diverse shapes of V1 simple cell receptive fields*. PLoS Comput Biol 7.10 (2011): e1002250.
- [6] Pietro Vertechi, Wieland Brendel, and Christian K. Machens. *Unsupervised learning of an efficient short-term memory network*. Advances in Neural Information Processing Systems 27 (2014).
- [7] John J. Hopfield. *Neural networks and physical systems with emergent collective computational abilities*. Proceedings of the National Academy of Sciences, 79.8 (1982): 2554–2558.
- [8] John Hertz, Richard G. Palmer, and Anders S. Krogh. *Introduction to the Theory of Neural Computation*. Perseus Publishing, 1991
- [9] Barak A. Pearlmutter. *Learning state space trajectories in recurrent neural networks*. Neural Computation, 1.2 (1989): 263–269.
- [10] David Susillo and Larry F. Abbott. *Generating coherent patterns of activity from chaotic neural networks*. Neuron, 63.4 (2009): 544–557.
- [11] Tim P. Vogels, Henning Sprekeler, Friedmann Zenke, Claudia Clopath, and Wulfram Gerstner. *Inhibitory plasticity balances excitation and inhibition in sensory pathways and memory networks*. Science, 334.6062 (2011):1569–1573.
- [12] Yin P, Fritz JB, Shamma SA. *Rapid spectrotemporal plasticity in primary auditory cortex during behavior*. J Neurosci. 2014 Mar 19;34(12):4396-408.
- [13] Mesgarani N, David SV, Fritz JB, Shamma SA. *Mechanisms of noise robust representation of speech in primary auditory cortex*. Proc Natl Acad Sci U S A. 2014 May 6;111(18):6792-7.
- [14] Pengsheng Zheng, Christos Dimitrakakis, and Jochen Triesch. *Network Self-Organization Explains the Statistics and Dynamics of Synaptic Connection Strengths in Cortex*. PLoS Comput Biol 9(01) (2013): e1002848

- [15] Andreea Lazar, Gordon Pipa, and Jochen Triesch. *SORN: A Self-Organizing Recurrent Neural Network*. *Frontiers in Computational Neuroscience* 3 (2009): 23
- [16] Wieland Brendel. *On the Structure and self-organized Formation of Neural Population Responses*. PhD Thesis, Ecole Normale Supérieure Paris
- [17] Aapo Hyvärinen, Juha Karhunen, and Erkki Oja. *Independent component analysis*. Wiley & Sons (2001).
- [18] Bruno A. Olshausen and David J. Field. *Sparse coding with an overcomplete basis set: A strategy employed by V1?* *Vision Research* 37.23 (1997):3311–3325.
- [19] Anthony J. Bell and Terrence J. Sejnowski. *The independent components of natural scenes are edge filters*. *Vision Research* 37.23 (1997): 3327–3338.
- [20] Ganguli Deep and Simoncelli P. Eero *Efficient sensory encoding and Bayesian inference with heterogeneous neural populations*. *Neural computation* (2014).
